# Supplementary material for: Linear stability analysis of transient electrodeposition in charged porous media: suppression of dendritic growth by surface conduction
Source: arXiv:1901.05033 ancillary file (2019-07-07)
Supplement: Supplementary file 1 [file supp.pdf]

# Linear stability analysis of transient electrodeposition in charged porous media: suppression of dendritic growth by surface conduction — supplementary material

Edwin Khoo,[1] Hongbo Zhao,[1] and Martin Z. Bazant[1,2,*]

[1]*Department of Chemical Engineering, Massachusetts Institute of Technology, Cambridge, Massachusetts 02139, USA*

[2]*Department of Mathematics, Massachusetts Institute of Technology, Cambridge, Massachusetts 02139, USA*

(Dated: May 23, 2019)

* Corresponding author: bazant@mit.edu

Throughout the supplementary material, to avoid cluttering the notation, we rewrite the (0) and (1) superscripts, which denote the base and perturbed states respectively in the main text, as 0 and 1 subscripts respectively. The "a" and "c" superscripts denote the anode and cathode respectively. We use subscripts to denote partial derivatives with respect to $x$ (with the exception that $u_x$ denotes the $x$ component of the moving reference frame velocity $u$), $y$, $z$ and $t$, primes to denote total derivatives with respect to $x$, and an overhead dot to denote the total derivative with respect to $t$.

## I. ELECTRODE/ELECTROLYTE INTERFACES

An illustration of the system under consideration is given in Figure 1 of the main text. In general, the electrode/electrolyte interfaces in 3D can be represented by $g^{\mathrm{a,c}}(x, y, z, t) = 0$ where $x \in [0, L_x]$, $y \in [0, L_y]$ and $z \in [0, L_z]$. If the electrode/electrolyte interfaces can be represented explicitly by $x = h^{\mathrm{a,c}}(y, z, t)$ where $h^{\mathrm{a,c}}$ is the electrode surface height, we express $g^{\mathrm{a,c}}(x, y, z, t)$ as $g^{\mathrm{a,c}}(x, y, z, t) = x - h^{\mathrm{a,c}}(y, z, t) = 0$. Thus [1, 2],

$$H = \left(1 + h_y^2 + h_z^2\right)^{\frac{1}{2}}, \tag{1}$$

$$\begin{aligned}\nabla_{\mathrm{s}} = \frac{1}{H^2}\Big\{&\big[\left(h_y^2 + h_z^2\right)e_x + h_y e_y + h_z e_z\big]\partial_x \\ &+ \big[h_y e_x + \left(h_z^2 + 1\right)e_y - h_y h_z e_z\big]\partial_y \\ &+ \big[h_z e_x - h_y h_z e_y + \left(h_y^2 + 1\right)e_z\big]\partial_z\Big\},\end{aligned} \tag{2}$$

$$\hat{n}(r = r_{\mathrm{m}}^{\mathrm{a}}) = -\frac{\nabla g^{\mathrm{a}}}{|\nabla g^{\mathrm{a}}|} = -\frac{e_x - h_y^{\mathrm{a}} e_y - h_z^{\mathrm{a}} e_z}{H^{\mathrm{a}}}, \tag{3}$$

$$\hat{n}(r = r_{\mathrm{m}}^{\mathrm{c}}) = \frac{\nabla g^{\mathrm{c}}}{|\nabla g^{\mathrm{c}}|} = \frac{e_x - h_y^{\mathrm{c}} e_y - h_z^{\mathrm{c}} e_z}{H^{\mathrm{c}}}, \tag{4}$$

$$\hat{n}(y = 0) = -e_y, \tag{5}$$

$$\hat{n}(y = L_y) = e_y, \tag{6}$$

$$\hat{n}(z = 0) = -e_z, \tag{7}$$

$$\hat{n}(z = L_z) = e_z, \tag{8}$$

$$2\mathscr{H}^{\mathrm{a}} = -\nabla_{\mathrm{s}} \cdot \hat{n}(r = r_{\mathrm{m}}^{\mathrm{a}}) = -\frac{1}{\left(H^{\mathrm{a}}\right)^3}\Big\{\big[\left(h_z^{\mathrm{a}}\right)^2 + 1\big]h_{yy}^{\mathrm{a}} - 2h_y^{\mathrm{a}} h_z^{\mathrm{a}} h_{yz}^{\mathrm{a}} + \Big[\left(h_y^{\mathrm{a}}\right)^2 + 1\Big]h_{zz}^{\mathrm{a}}\Big\}, \tag{9}$$

$$2\mathscr{H}^{\mathrm{c}} = -\nabla_{\mathrm{s}} \cdot \hat{n}(r = r_{\mathrm{m}}^{\mathrm{c}}) = \frac{1}{\left(H^{\mathrm{c}}\right)^{3}} \left\{ \left[ \left(h_z^{\mathrm{c}}\right)^2 + 1 \right] h_{yy}^{\mathrm{c}} - 2 h_y^{\mathrm{c}} h_z^{\mathrm{c}} h_{yz}^{\mathrm{c}} + \left[ \left(h_y^{\mathrm{c}}\right)^2 + 1 \right] h_{zz}^{\mathrm{c}} \right\}, \tag{10}$$

$$v_{\mathrm{I}} = \epsilon_{\mathrm{p}} \dot{r}_{\mathrm{m}} = \epsilon_{\mathrm{p}} [(h_t + h_y \dot{y} + h_z \dot{z}) e_x + \dot{y} e_y + \dot{z} e_z], \tag{11}$$

$$v_{\mathrm{In}}^{\mathrm{a}} = \hat{n} \cdot v_{\mathrm{I}}(r = r_{\mathrm{m}}^{\mathrm{a}}) = -\frac{\epsilon_{\mathrm{p}}}{H^{\mathrm{a}}} h_t^{\mathrm{a}}, \tag{12}$$

$$v_{\mathrm{In}}^{\mathrm{c}} = \hat{n} \cdot v_{\mathrm{I}}(r = r_{\mathrm{m}}^{\mathrm{c}}) = \frac{\epsilon_{\mathrm{p}}}{H^{\mathrm{c}}} h_t^{\mathrm{c}}, \tag{13}$$

where $r = [x, y, z]^{\mathrm{T}}$ is the position vector, $r_{\mathrm{m}}^{\mathrm{a,c}} = [x_{\mathrm{m}}^{\mathrm{a,c}}, y_{\mathrm{m}}^{\mathrm{a,c}}, z_{\mathrm{m}}^{\mathrm{a,c}}]^{\mathrm{T}}$, $\mathscr{H}^{\mathrm{a,c}}$, $v_{\mathrm{I}}^{\mathrm{a,c}}$ and $v_{\mathrm{In}}^{\mathrm{a,c}}$ are the position, mean curvature, velocity and normal velocity of the electrode/electrolyte interface respectively, $\nabla_{\mathrm{s}}$ is the surface gradient operator and $\hat{n}(r = r_{\mathrm{m}}^{\mathrm{a,c}})$ is the unit normal that points outwards from the electrolyte. We let $k = [k_y, k_z]^{\mathrm{T}}$ and $\xi = [y, z]^{\mathrm{T}}$ where $k$ is the wavevector, and $k_y$ and $k_z$ are the wavenumbers in the $y$ and $z$ directions respectively. Therefore, $k \cdot \xi = k_y y + k_z z$, $k^2 = \|k\|_2^2 = k_y^2 + k_z^2$ where $\|\cdot\|_2$ is the $L^2$-norm and $\|k\|_2$ is the overall wavenumber, and the wavelength $\lambda$ is given by $\lambda = \frac{2\pi}{\|k\|_2}$. For brevity, we write the overall wavenumber as $k$ and it is obvious from context whether $k$ refers to the wavevector or overall wavenumber. We assume that the perturbations to the electrode/electrolyte interfaces are sinusoidal in the $y$ and $z$ directions given by

$$h(\xi, t) = h_0(t) + \epsilon \Re[h_1 \exp(ik \cdot \xi + \omega t)] + \mathcal{O}\left(\epsilon^2\right) \tag{14}$$

where $\epsilon \ll 1$ is a dimensionless small parameter, the 0 and 1 subscripts denote the base and perturbed states respectively, $\Re(\cdot)$ gives the real part of a complex number, $h_1$ is the complex-valued perturbation amplitude of the electrode surface height, and $\omega$ is the complex-valued growth rate of the perturbation.

For nondimensionalization, we define $\tilde{x} \equiv \frac{x}{L_x}$, $\tilde{y} \equiv \frac{y}{L_x}$, $\tilde{z} \equiv \frac{z}{L_x}$, $\tilde{t} \equiv \frac{D_{\mathrm{amb0}} t}{L_x^2}$, $\tilde{L}_y \equiv \frac{L_y}{L_x}$, $\tilde{L}_z \equiv \frac{L_z}{L_x}$, $\tilde{r} \equiv \frac{r}{L_x}$, $\tilde{r}_{\mathrm{m}}^{\mathrm{a,c}} \equiv \frac{r_{\mathrm{m}}^{\mathrm{a,c}}}{L_x}$, $\tilde{\nabla} \equiv L_x \nabla$, $\tilde{\mathscr{H}}^{\mathrm{a,c}} \equiv L_x \mathscr{H}^{\mathrm{a,c}}$, $\tilde{v}_{\mathrm{I}}^{\mathrm{a,c}} \equiv \frac{L_x v_{\mathrm{I}}^{\mathrm{a,c}}}{\epsilon_{\mathrm{p}} D_{\mathrm{amb0}}}$, $\tilde{v}_{\mathrm{In}}^{\mathrm{a,c}} \equiv \frac{L_x v_{\mathrm{In}}^{\mathrm{a,c}}}{\epsilon_{\mathrm{p}} D_{\mathrm{amb0}}}$, $\tilde{h}^{\mathrm{a,c}} \equiv \frac{h^{\mathrm{a,c}}}{L_x}$, $\tilde{h}_0 \equiv \frac{h_0}{L_x}$, $\tilde{h}_1 \equiv \frac{h_1}{L_x}$, $\tilde{k}_y \equiv L_x k_y$, $\tilde{k}_z \equiv L_x k_z$, $\tilde{k} \equiv L_x k$, $\tilde{\lambda} \equiv \frac{\lambda}{L_x}$, $\tilde{\xi} \equiv \frac{\xi}{L_x}$ and $\tilde{\omega} \equiv \frac{L_x^2 \omega}{D_{\mathrm{amb0}}}$. Therefore, dropping tildes on dimensionless variables and parameters to avoid cluttering the notation,

$$H = \left(1 + h_y^2 + h_z^2\right)^{\frac{1}{2}}, \tag{15}$$

$$\hat{n}(r = r_{\mathrm{m}}^{\mathrm{a}}) = -\frac{e_x - h_y^{\mathrm{a}} e_y - h_z^{\mathrm{a}} e_z}{H^{\mathrm{a}}}, \tag{16}$$

$$\hat{n}(r = r_{\mathrm{m}}^{\mathrm{c}}) = \frac{e_x - h_y^{\mathrm{c}} e_y - h_z^{\mathrm{c}} e_z}{H^{\mathrm{c}}}, \tag{17}$$

$$\hat{n}(y=0) = -e_y, \tag{18}$$

$$\hat{n}(y=L_y) = e_y, \tag{19}$$

$$\hat{n}(z=0) = -e_z, \tag{20}$$

$$\hat{n}(z=L_z) = e_z, \tag{21}$$

$$2\mathscr{H}^{\mathrm{a}} = -\frac{1}{(H^{\mathrm{a}})^3}\Big\{\big[(h_z^{\mathrm{a}})^2+1\big]h_{yy}^{\mathrm{a}} - 2h_y^{\mathrm{a}}h_z^{\mathrm{a}}h_{yz}^{\mathrm{a}} + \Big[\big(h_y^{\mathrm{a}}\big)^2+1\Big]h_{zz}^{\mathrm{a}}\Big\}, \tag{22}$$

$$2\mathscr{H}^{\mathrm{c}} = \frac{1}{(H^{\mathrm{c}})^3}\Big\{\big[(h_z^{\mathrm{c}})^2+1\big]h_{yy}^{\mathrm{c}} - 2h_y^{\mathrm{c}}h_z^{\mathrm{c}}h_{yz}^{\mathrm{c}} + \Big[\big(h_y^{\mathrm{c}}\big)^2+1\Big]h_{zz}^{\mathrm{c}}\Big\}, \tag{23}$$

$$v_{\mathrm{In}}^{\mathrm{a}} = -\frac{1}{H^{\mathrm{a}}}h_t^{\mathrm{a}}, \tag{24}$$

$$v_{\mathrm{In}}^{\mathrm{c}} = \frac{1}{H^{\mathrm{c}}}h_t^{\mathrm{c}}, \tag{25}$$

$$h(\xi,t) = h_0(t) + \epsilon\Re[h_1\exp(ik\cdot\xi+\omega t)] + \mathcal{O}\big(\epsilon^2\big). \tag{26}$$

## II. DIMENSIONLESS FULL MODEL

We define more dimensionless variables and parameters in order to nondimensionalize the full model: $\tilde{c}_\pm \equiv \frac{c_\pm}{\nu_\pm c_0}$, $\tilde{\beta}_1 \equiv \frac{\beta_1}{\nu_- c_0} = 1 + \frac{\tilde{\rho}_{\mathrm{s}}+|\tilde{\rho}_{\mathrm{s}}|}{2}$, $\tilde{\phi} \equiv \frac{e\phi}{k_{\mathrm{B}}T}$, $\tilde{F}_\pm \equiv \frac{L_x F_\pm}{\epsilon_{\mathrm{p}} D_{\mathrm{amb0}}\nu_\pm c_0}$, $\tilde{D}_{\pm 0} \equiv \frac{D_{\pm 0}}{D_{\mathrm{amb0}}}$, $\tilde{J} \equiv \frac{J}{J_{\mathrm{lim}}}$, $\tilde{I} \equiv \frac{I}{I_{\mathrm{lim}}}$, $\tilde{\rho}_{\mathrm{s}} \equiv \frac{\rho_{\mathrm{s}}}{z_+\nu_+ e c_0} = -\frac{\rho_{\mathrm{s}}}{z_-\nu_- e c_0}$, $\tilde{j}_0 \equiv \frac{\epsilon_{\mathrm{p}} j_0}{J_{\mathrm{lim}}}$, $\tilde{J}_{\mathrm{F}} \equiv \frac{\epsilon_{\mathrm{p}} J_{\mathrm{F}}}{J_{\mathrm{lim}}}$, $\tilde{k}_0 \equiv \frac{e\epsilon_{\mathrm{p}} k_0}{J_{\mathrm{lim}}}$, $\tilde{\gamma} \equiv \frac{\Omega\gamma}{L_x k_{\mathrm{B}} T}$, $\tilde{u} \equiv \frac{L_x u}{\epsilon_{\mathrm{p}} D_{\mathrm{amb0}}}$, $\tilde{u}_x \equiv \frac{L_x u_x}{\epsilon_{\mathrm{p}} D_{\mathrm{amb0}}}$, $\beta_{\mathrm{D}} = -\frac{z_- D_{-0}}{2(z_+ D_{+0} - z_- D_{-0})}$, $\beta_{\mathrm{m}} = \nu_+ c_0 \Omega$, $\beta_{\mathrm{v}} = \frac{\beta_{\mathrm{m}}}{\beta_{\mathrm{D}}}$, $\xi_+ = \frac{\nu_+ c_0}{c_+^\ominus}$, $\mathrm{Da} = \tilde{k}_0 = \frac{e\epsilon_{\mathrm{p}} k_0}{J_{\mathrm{lim}}}$ and $\mathrm{Ca} = \tilde{\gamma} = \frac{\Omega\gamma}{L_x k_{\mathrm{B}} T}$ where we note that $I_{\mathrm{lim}} = J_{\mathrm{lim}} A$ and $A = L_y L_z$. To avoid cluttering the notation, we drop tildes on all dimensionless variables and parameters, the 0 subscript for diffusivities and the $-$ subscript for anion-related variables and parameters in all following sections unless otherwise stated. Recall that we have picked a moving reference frame with a velocity $u(t) = u_x(t)e_x$ such that the average positions of the dissolving anode and growing cathode remain stationary. The dimensionless governing PDEs (partial differential equations) are

$$\frac{\partial c}{\partial t} + \nabla\cdot F = 0, \quad F = -D(\nabla c + zc\nabla\phi), \tag{27}$$

$$\nabla\cdot J = 0, \quad J = \beta_{\mathrm{D}}\{(D-D_+)\nabla c + [z_+ D_+ \rho_{\mathrm{s}} - (z_+ D_+ - zD)c]\nabla\phi\}, \tag{28}$$

$$\rho_{\mathrm{s}} = c - c_+. \tag{29}$$

The dimensionless Faradaic current density $J_{\mathrm{F}}$ is

$$J_{\mathrm{F}} = j_0\{\exp(-\alpha n\eta) - \exp[(1-\alpha)n\eta]\}, \tag{30}$$

$$j_0 = \mathrm{Da}n[\xi_+(c-\rho_\mathrm{s})]^{1-\alpha}, \tag{31}$$

$$\eta = \Delta\phi - \Delta\phi^\mathrm{eq}, \tag{32}$$

$$\Delta\phi = \phi_\mathrm{e} - \phi, \tag{33}$$

$$\Delta\phi^\mathrm{eq} = \frac{1}{n}\ln[\xi_+(c-\rho_\mathrm{s})] + E^\Theta - \frac{2\gamma\mathscr{H}}{n}. \tag{34}$$

The dimensionless boundary conditions are

$$\phi_\mathrm{e}^\mathrm{a} = 0, \tag{35}$$

$$\hat{n}\cdot F(r = r_\mathrm{m}^\mathrm{a,c}) = 0, \tag{36}$$

$$\hat{n}\cdot J(r = r_\mathrm{m}^\mathrm{a,c}) = J_\mathrm{F}^\mathrm{a,c}, \tag{37}$$

$$\hat{n}\cdot F(r = r_\mathrm{other}) = 0, \tag{38}$$

$$\hat{n}\cdot J(r = r_\mathrm{other}) = 0, \tag{39}$$

$$v_\mathrm{In}^\mathrm{a,c} = -\beta_\mathrm{v}\hat{n}\cdot J(r = r_\mathrm{m}^\mathrm{a,c}) - \hat{n}\cdot u(r = r_\mathrm{m}^\mathrm{a,c}). \tag{40}$$

For galvanostatic conditions,

$$\int \hat{n}\cdot J(r = r_\mathrm{m}^\mathrm{c})\,\mathrm{d}S^\mathrm{c} = \int -\hat{n}\cdot J(r = r_\mathrm{m}^\mathrm{a})\,\mathrm{d}S^\mathrm{a} = I_\mathrm{a}. \tag{41}$$

For potentiostatic conditions,

$$\phi_\mathrm{e}^\mathrm{c} = V. \tag{42}$$

The dimensionless initial conditions are

$$c(t=0) = \beta_1, \tag{43}$$

$$x_\mathrm{m}^\mathrm{a}(t=0) = 0, \tag{44}$$

$$x_\mathrm{m}^\mathrm{c}(t=0) = 1. \tag{45}$$

## III. EQUATIONS FOR BASE AND PERTURBED STATES

We derive the perturbation expressions in Sections III A, III B, III C and III D. We then substitute these expressions into the full model in Section II and match the $\mathcal{O}(1)$ (base state) and $\mathcal{O}(\epsilon)$ (perturbed state) terms. The equations for the base state are given in Section III E and that for the perturbed state are given in Section III F. The goal of the linear stability analysis is to solve the equations at $\mathcal{O}(1)$ and $\mathcal{O}(\epsilon)$ and compute the dimensionless dispersion

relation $\omega(k)$. In general, $\omega$ is complex-valued. If $\max\{\Re(\omega)\} < 0$, we conclude that the base state is linearly stable and if $\max\{\Re(\omega)\} > 0$, we conclude that the base state is linearly unstable. However, if $\max\{\Re(\omega)\} = 0$, the base state is marginally stable.

### A. Perturbations and linearization

In response to the perturbations to the electrode/electrolyte interfaces, we assume that the perturbations to the field variables $c$ and $\phi$ are similarly given by

$$c(x,\xi,t) = c_0(x,t) + \epsilon\Re[c_1(x)\exp(ik\cdot\xi + \omega t)] + \mathcal{O}(\epsilon^2), \tag{46}$$

$$\phi(x,\xi,t) = \phi_0(x,t) + \epsilon\Re[\phi_1(x)\exp(ik\cdot\xi + \omega t)] + \mathcal{O}(\epsilon^2), \tag{47}$$

where $c_1$ and $\phi_1$ are the complex-valued perturbation amplitudes of anion concentration and electrolyte electric potential respectively. For brevity, we let $\hat{\epsilon} = \epsilon\exp(ik\cdot\xi + \omega t)$ and $\theta \in \{c,\phi\}$. We also drop $\Re(\cdot)$ with the understanding that we are only interested in the real parts of complex-valued variables. Therefore,

$$h(\xi,t) = h_0(t) + \hat{\epsilon}h_1 + \mathcal{O}(\epsilon^2), \tag{48}$$

$$\theta(x,\xi,t) = \theta_0(x,t) + \hat{\epsilon}\theta_1(x) + \mathcal{O}(\epsilon^2). \tag{49}$$

The required temporal and spatial derivatives are given by

$$h_t = \dot{h}_0 + \hat{\epsilon}\omega h_1 + \mathcal{O}(\epsilon^2), \tag{50}$$

$$h_y = \hat{\epsilon}ik_y h_1 + \mathcal{O}(\epsilon^2), \quad h_z = \hat{\epsilon}ik_z h_1 + \mathcal{O}(\epsilon^2), \tag{51}$$

$$h_{yy} = -\hat{\epsilon}k_y^2 h_1 + \mathcal{O}(\epsilon^2), \quad h_{zz} = -\hat{\epsilon}k_z^2 h_1 + \mathcal{O}(\epsilon^2), \quad h_{yz} = -\hat{\epsilon}k_y k_z h_1 + \mathcal{O}(\epsilon^2), \tag{52}$$

$$\theta_t = \theta_{0,t} + \hat{\epsilon}\omega\theta_1 + \mathcal{O}(\epsilon^2), \tag{53}$$

$$\theta_x = \theta_{0,x} + \hat{\epsilon}\theta_1' + \mathcal{O}(\epsilon^2), \tag{54}$$

$$\theta_{xx} = \theta_{0,xx} + \hat{\epsilon}\theta_1'' + \mathcal{O}(\epsilon^2), \tag{55}$$

$$\theta_y = \hat{\epsilon}ik_y\theta_1 + \mathcal{O}(\epsilon^2), \quad \theta_z = \hat{\epsilon}ik_z\theta_1 + \mathcal{O}(\epsilon^2), \tag{56}$$

$$\theta_{yy} = -\hat{\epsilon}k_y^2\theta_1 + \mathcal{O}(\epsilon^2), \quad \theta_{zz} = -\hat{\epsilon}k_z^2\theta_1 + \mathcal{O}(\epsilon^2), \tag{57}$$

$$c\phi_x = c_0\phi_{0,x} + \hat{\epsilon}(c_0\phi_1' + \phi_{0,x}c_1) + \mathcal{O}(\epsilon^2), \tag{58}$$

$$(c\phi_x)_x = (c_0\phi_{0,x})_x + \hat{\epsilon}(c_0\phi_1' + \phi_{0,x}c_1)_x + \mathcal{O}(\epsilon^2), \tag{59}$$

$$c\phi_y = \hat{\epsilon}ik_y c_0\phi_1 + \mathcal{O}(\epsilon^2), \quad c\phi_z = \hat{\epsilon}ik_z c_0\phi_1 + \mathcal{O}(\epsilon^2), \tag{60}$$

$$(c\phi_y)_y = -\hat{\epsilon}k_y^2 c_0\phi_1 + \mathcal{O}(\epsilon^2), \quad (c\phi_z)_z = -\hat{\epsilon}k_z^2 c_0\phi_1 + \mathcal{O}(\epsilon^2), \tag{61}$$

$$H^{-1} = 1 + \mathcal{O}(\epsilon^2), \tag{62}$$

$$H^{-3} = 1 + \mathcal{O}(\epsilon^2), \tag{63}$$

$$\hat{n}(r = r_{\mathrm{m}}^{\mathrm{a}}) = -\left\{\left[1 + \mathcal{O}(\epsilon^2)\right]e_x - \left[\hat{\epsilon}ik_y h_1^{\mathrm{a}} + \mathcal{O}(\epsilon^2)\right]e_y - \left[\hat{\epsilon}ik_z h_1^{\mathrm{a}} + \mathcal{O}(\epsilon^2)\right]e_z\right\}, \tag{64}$$

$$\hat{n}(r = r_{\mathrm{m}}^{\mathrm{c}}) = \left[1 + \mathcal{O}(\epsilon^2)\right]e_x - \left[\hat{\epsilon}ik_y h_1^{\mathrm{c}} + \mathcal{O}(\epsilon^2)\right]e_y - \left[\hat{\epsilon}ik_z h_1^{\mathrm{c}} + \mathcal{O}(\epsilon^2)\right]e_z, \tag{65}$$

$$2\mathscr{H}^{\mathrm{a}} = \hat{\epsilon}k^2 h_1^{\mathrm{a}} + \mathcal{O}(\epsilon^2), \tag{66}$$

$$2\mathscr{H}^{\mathrm{c}} = -\hat{\epsilon}k^2 h_1^{\mathrm{c}} + \mathcal{O}(\epsilon^2), \tag{67}$$

$$v_{\mathrm{In}}^{\mathrm{a}} = -\left(\dot{h}_0^{\mathrm{a}} + \hat{\epsilon}\omega h_1^{\mathrm{a}}\right) + \mathcal{O}(\epsilon^2), \tag{68}$$

$$v_{\mathrm{In}}^{\mathrm{c}} = \dot{h}_0^{\mathrm{c}} + \hat{\epsilon}\omega h_1^{\mathrm{c}} + \mathcal{O}(\epsilon^2). \tag{69}$$

### B. Expressions in domain

For brevity, we stop writing $\mathcal{O}(\epsilon^2)$. In the domain,

$$\nabla^2\theta = \theta_{xx} + \theta_{yy} + \theta_{zz} = \theta_{0,xx} + \hat{\epsilon}\left(\theta_1'' - k^2\theta_1\right), \tag{70}$$

$$\nabla\cdot(c\nabla\phi) = (c\phi_x)_x + (c\phi_y)_y + (c\phi_z)_z = (c_0\phi_{0,x})_x + \hat{\epsilon}\left[(c_0\phi_1' + \phi_{0,x}c_1)_x - k^2 c_0\phi_1\right], \tag{71}$$

$$\nabla\cdot F = -D\left[\nabla^2 c + z\nabla\cdot(c\nabla\phi)\right] = \nabla\cdot F_0 + \hat{\epsilon}\nabla\cdot F_1, \tag{72}$$

$$\nabla\cdot F_0 = -D\left[c_{0,xx} + z(c_0\phi_{0,x})_x\right], \tag{73}$$

$$\nabla\cdot F_1 = -D\left\{c_1'' - k^2 c_1 + z\left[(c_0\phi_1' + \phi_{0,x}c_1)_x - k^2 c_0\phi_1\right]\right\}, \tag{74}$$

$$\nabla\cdot J = \beta_{\mathrm{D}}\left[(D - D_+)\nabla^2 c + z_+D_+\rho_{\mathrm{s}}\nabla^2\phi - (z_+D_+ - zD)\nabla\cdot(c\nabla\phi)\right] = \nabla\cdot J_0 + \hat{\epsilon}\nabla\cdot J_1, \tag{75}$$

$$\nabla\cdot J_0 = \beta_{\mathrm{D}}\left[(D - D_+)c_{0,xx} + z_+D_+\rho_{\mathrm{s}}\phi_{0,xx} - (z_+D_+ - zD)(c_0\phi_{0,x})_x\right], \tag{76}$$

$$\nabla\cdot J_1 = \beta_{\mathrm{D}}\left\{(D - D_+)\left(c_1'' - k^2 c_1\right) + z_+D_+\rho_{\mathrm{s}}\left(\phi_1'' - k^2\phi_1\right) - (z_+D_+ - zD)\left[(c_0\phi_1' + \phi_{0,x}c_1)_x - k^2 c_0\phi_1\right]\right\}. \tag{77}$$

### C. Expressions at boundaries

To evaluate $\theta$, $\nabla\theta$ and $\hat{n}\cdot\theta$ at the electrode/electrolyte interface at $x = h$, we require their Taylor series expansions around the base electrode/electrolyte interface at $x = h_0$. We

first note that

$$h - h_0 = \hat{\epsilon} h_1 + \mathcal{O}\big(\epsilon^2\big), \tag{78}$$

$$|h - h_0| = \big|\hat{\epsilon} h_1 + \mathcal{O}\big(\epsilon^2\big)\big| = \mathcal{O}(\epsilon), \tag{79}$$

$$|h - h_0|^2 = \big|\hat{\epsilon} h_1 + \mathcal{O}\big(\epsilon^2\big)\big|^2 = \mathcal{O}\big(\epsilon^2\big). \tag{80}$$

For brevity, we stop writing $\mathcal{O}(\epsilon^2)$. Therefore, performing the Taylor series expansion of $\theta$ around $x = h_0$,

$$\begin{aligned}\theta(x = h) &= \theta_0(x = h) + \hat{\epsilon}\theta_1(x = h)\\ &= \theta_0(x = h_0) + \theta_{0,x}(x = h_0)(h - h_0) + \hat{\epsilon}\theta_1(x = h_0)\\ &= \theta_0(x = h_0) + \hat{\epsilon}[h_1\theta_{0,x}(x = h_0) + \theta_1(x = h_0)].\end{aligned} \tag{81}$$

To avoid cluttering the notation, we stop writing $x = h$ and $x = h_0$ since it is obvious from context where the evaluations should be performed. Therefore, at both the anode and cathode,

$$\theta = \theta_0 + \hat{\epsilon}(h_1\theta_{0,x} + \theta_1), \tag{82}$$

$$\theta_x = \theta_{0,x} + \hat{\epsilon}(h_1\theta_{0,xx} + \theta_1'), \tag{83}$$

$$\theta_y = \hat{\epsilon} i k_y \theta_1, \quad \theta_z = \hat{\epsilon} i k_z \theta_1, \tag{84}$$

$$c\phi_x = c_0\phi_{0,x} + \hat{\epsilon}\big[h_1(c_0\phi_{0,x})_x + c_0\phi_1' + \phi_{0,x}c_1\big], \tag{85}$$

$$c\phi_y = \hat{\epsilon} i k_y c_0\phi_1, \quad c\phi_z = \hat{\epsilon} i k_z c_0\phi_1, \tag{86}$$

$$\nabla\theta = \theta_x e_x + \theta_y e_y + \theta_z e_z, \tag{87}$$

$$c\nabla\phi = c\phi_x e_x + c\phi_y e_y + c\phi_z e_z. \tag{88}$$

At the anode,

$$\hat{n}\cdot\nabla\theta = -\theta_x = -[\theta_{0,x} + \hat{\epsilon}(h_1\theta_{0,xx} + \theta_1')], \tag{89}$$

$$\hat{n}\cdot(c\nabla\phi) = -c\phi_x = -\big\{c_0\phi_{0,x} + \hat{\epsilon}\big[h_1(c_0\phi_{0,x})_x + c_0\phi_1' + \phi_{0,x}c_1\big]\big\}, \tag{90}$$

$$\hat{n}\cdot F = -D\hat{n}\cdot(\nabla c + zc\nabla\phi) = \hat{n}\cdot F_0 + \hat{\epsilon}\hat{n}\cdot F_1, \tag{91}$$

$$\hat{n}\cdot F_0 = -D(-c_{0,x} - zc_0\phi_{0,x}), \tag{92}$$

$$\hat{n}\cdot F_1 = -D\big\{-h_1c_{0,xx} - c_1' - z\big[h_1(c_0\phi_{0,x})_x + c_0\phi_1' + \phi_{0,x}c_1\big]\big\}, \tag{93}$$

$$\hat{n}\cdot J = \beta_{\mathrm{D}}\hat{n}\cdot[(D - D_+)\nabla c + z_+D_+\rho_{\mathrm{s}}\nabla\phi - (z_+D_+ - zD)c\nabla\phi] = \hat{n}\cdot J_0 + \hat{\epsilon}\hat{n}\cdot J_1, \tag{94}$$

$$\hat{n}\cdot J_0 = \beta_{\rm D}[-(D-D_+)c_{0,x} - z_+D_+\rho_{\rm s}\phi_{0,x} + (z_+D_+ - zD)c_0\phi_{0,x}], \tag{95}$$

$$\hat{n}\cdot J_1 = \beta_{\rm D}\{-(D-D_+)(h_1c_{0,xx}+c_1') - z_+D_+\rho_{\rm s}(h_1\phi_{0,xx}+\phi_1') + (z_+D_+ - zD)\big[h_1(c_0\phi_{0,x})_x + c_0\phi_1' + \phi_{0,x}c_1\big]\}, \tag{96}$$

$$\hat{n}\cdot u = -u_x. \tag{97}$$

For the electrochemical reaction kinetics,

$$\Delta\phi = \phi_{\rm e} - \phi_0 - \hat{\epsilon}(h_1\phi_{0,x}+\phi_1), \tag{98}$$

$$\Delta\phi^{\rm eq} = \frac{1}{n}\ln[\xi_+(c_0-\rho_{\rm s})] + E^\Theta + \hat{\epsilon}\left[\frac{1}{n}\left(\frac{h_1c_{0,x}+c_1}{c_0-\rho_{\rm s}} - \gamma k^2h_1\right)\right], \tag{99}$$

$$\eta = \eta_0 + \hat{\epsilon}\eta_1, \tag{100}$$

$$\eta_0 = \phi_{\rm e} - \phi_0 - \frac{1}{n}\ln[\xi_+(c_0-\rho_{\rm s})] - E^\Theta, \tag{101}$$

$$\eta_1 = -(h_1\phi_{0,x}+\phi_1) - \frac{1}{n}\left(\frac{h_1c_{0,x}+c_1}{c_0-\rho_{\rm s}} - \gamma k^2h_1\right), \tag{102}$$

$$j_0 = j_{0,0} + \hat{\epsilon}j_{0,1}, \tag{103}$$

$$j_{0,0} = {\rm Da}n[\xi_+(c_0-\rho_{\rm s})]^{1-\alpha}, \tag{104}$$

$$j_{0,1} = j_{0,0}\frac{(1-\alpha)(h_1c_{0,x}+c_1)}{c_0-\rho_{\rm s}}, \tag{105}$$

$$J_{\rm F} = J_{\rm F,0} + \hat{\epsilon}J_{\rm F,1}, \tag{106}$$

$$J_{\rm F,0} = j_{0,0}\{\exp(-\alpha n\eta_0) - \exp[(1-\alpha)n\eta_0]\}, \tag{107}$$

$$J_{\rm F,1} = j_{0,0}\left\{[-\alpha\exp(-\alpha n\eta_0) - (1-\alpha)\exp[(1-\alpha)n\eta_0]]n\eta_1 + [\exp(-\alpha n\eta_0) - \exp[(1-\alpha)n\eta_0]]\frac{(1-\alpha)(h_1c_{0,x}+c_1)}{c_0-\rho_{\rm s}}\right\}. \tag{108}$$

The signs of the expressions involving $\hat{n}$, including $\mathscr{H}$ and $v_{\rm In}$, at the cathode are opposite to that at the anode. Therefore, at the cathode,

$$\hat{n}\cdot\nabla\theta = \theta_x = \theta_{0,x} + \hat{\epsilon}(h_1\theta_{0,xx}+\theta_1'), \tag{109}$$

$$\hat{n}\cdot(c\nabla\phi) = c\phi_x = c_0\phi_{0,x} + \hat{\epsilon}\big[h_1(c_0\phi_{0,x})_x + c_0\phi_1' + \phi_{0,x}c_1\big], \tag{110}$$

$$\hat{n}\cdot F = -D\hat{n}\cdot(\nabla c + zc\nabla\phi) = \hat{n}\cdot F_0 + \hat{\epsilon}\hat{n}\cdot F_1, \tag{111}$$

$$\hat{n}\cdot F_0 = -D(c_{0,x} + zc_0\phi_{0,x}), \tag{112}$$

$$\hat{n}\cdot F_1 = -D\big\{h_1c_{0,xx} + c_1' + z\big[h_1(c_0\phi_{0,x})_x + c_0\phi_1' + \phi_{0,x}c_1\big]\big\}, \tag{113}$$

$$\hat{n}\cdot J = \beta_{\rm D}\hat{n}\cdot[(D-D_+)\nabla c + z_+D_+\rho_{\rm s}\nabla\phi - (z_+D_+ - zD)c\nabla\phi] = \hat{n}\cdot J_0 + \hat{\epsilon}\hat{n}\cdot J_1, \tag{114}$$

$$\hat{n} \cdot J_0 = \beta_\mathrm{D}[(D - D_+)c_{0,x} + z_+ D_+ \rho_\mathrm{s} \phi_{0,x} - (z_+ D_+ - zD)c_0 \phi_{0,x}], \tag{115}$$

$$\hat{n} \cdot J_1 = \beta_\mathrm{D}\{(D - D_+)(h_1 c_{0,xx} + c_1') + z_+ D_+ \rho_\mathrm{s}(h_1 \phi_{0,xx} + \phi_1') - (z_+ D_+ - zD)\big[h_1 (c_0 \phi_{0,x})_x + c_0 \phi_1' + \phi_{0,x} c_1\big]\big\}, \tag{116}$$

$$\hat{n} \cdot u = u_x. \tag{117}$$

For the electrochemical reaction kinetics,

$$\Delta\phi = \phi_\mathrm{e} - \phi_0 - \hat{\epsilon}(h_1 \phi_{0,x} + \phi_1), \tag{118}$$

$$\Delta\phi^\mathrm{eq} = \frac{1}{n}\ln[\xi_+(c_0 - \rho_\mathrm{s})] + E^\Theta + \hat{\epsilon}\left[\frac{1}{n}\left(\frac{h_1 c_{0,x} + c_1}{c_0 - \rho_\mathrm{s}} + \gamma k^2 h_1\right)\right], \tag{119}$$

$$\eta = \eta_0 + \hat{\epsilon}\eta_1, \tag{120}$$

$$\eta_0 = \phi_\mathrm{e} - \phi_0 - \frac{1}{n}\ln[\xi_+(c_0 - \rho_\mathrm{s})] - E^\Theta, \tag{121}$$

$$\eta_1 = -(h_1 \phi_{0,x} + \phi_1) - \frac{1}{n}\left(\frac{h_1 c_{0,x} + c_1}{c_0 - \rho_\mathrm{s}} + \gamma k^2 h_1\right), \tag{122}$$

$$j_0 = j_{0,0} + \hat{\epsilon} j_{0,1}, \tag{123}$$

$$j_{0,0} = \mathrm{Da} n[\xi_+(c_0 - \rho_\mathrm{s})]^{1-\alpha}, \tag{124}$$

$$j_{0,1} = j_{0,0}\frac{(1-\alpha)(h_1 c_{0,x} + c_1)}{c_0 - \rho_\mathrm{s}}, \tag{125}$$

$$J_\mathrm{F} = J_{\mathrm{F},0} + \hat{\epsilon} J_{\mathrm{F},1}, \tag{126}$$

$$J_{\mathrm{F},0} = j_{0,0}\{\exp(-\alpha n \eta_0) - \exp[(1-\alpha)n\eta_0]\}, \tag{127}$$

$$J_{\mathrm{F},1} = j_{0,0}\Big\{[-\alpha \exp(-\alpha n \eta_0) - (1-\alpha)\exp[(1-\alpha)n\eta_0]]n\eta_1 + [\exp(-\alpha n \eta_0) - \exp[(1-\alpha)n\eta_0]]\frac{(1-\alpha)(h_1 c_{0,x} + c_1)}{c_0 - \rho_\mathrm{s}}\Big\}. \tag{128}$$

We can rewrite $J_{\mathrm{F},1}$ in a more physically interpretable fashion by first defining the following dimensionless variables

$$\alpha_3 = -\alpha \exp(-\alpha n \eta_0) - (1-\alpha)\exp[(1-\alpha)n\eta_0] = \frac{1}{n}\frac{\partial \alpha_4}{\partial \eta_0}, \tag{129}$$

$$\alpha_4 = \exp(-\alpha n \eta_0) - \exp[(1-\alpha)n\eta_0]. \tag{130}$$

Therefore, at the anode,

$$J_{\mathrm{F},1} = j_{0,0}\Big(\hat{D}_1 h_1 + \hat{D}_2 c_1 + \hat{D}_3 \phi_1\Big), \tag{131}$$

$$\hat{D}_1 = \alpha_3 n\left(-\phi_{0,x} + \frac{\gamma k^2}{n}\right) + \frac{\exp(-\alpha n \eta_0) c_{0,x}}{c_0 - \rho_\mathrm{s}}, \tag{132}$$

$$\hat{D}_2 = \frac{\exp(-\alpha n\eta_0)}{c_0 - \rho_\mathrm{s}}, \tag{133}$$

$$\hat{D}_3 = -\alpha_3 n, \tag{134}$$

and at the cathode,

$$J_{\mathrm{F},1} = j_{0,0}\Big(\hat{G}_1 h_1 + \hat{G}_2 c_1 + \hat{G}_3 \phi_1\Big), \tag{135}$$

$$\hat{G}_1 = \alpha_3 n\left(-\phi_{0,x} - \frac{\gamma k^2}{n}\right) + \frac{\exp(-\alpha n\eta_0)c_{0,x}}{c_0 - \rho_\mathrm{s}}, \tag{136}$$

$$\hat{G}_2 = \frac{\exp(-\alpha n\eta_0)}{c_0 - \rho_\mathrm{s}}, \tag{137}$$

$$\hat{G}_3 = -\alpha_3 n. \tag{138}$$

At the boundaries at $r = r_\mathrm{other}$, because of the $\hat{n}\cdot F(r = r_\mathrm{other}) = 0$ and $\hat{n}\cdot J(r = r_\mathrm{other}) = 0$ boundary conditions, we require $\theta_y(y = 0) = \theta_y(y = L_y) = 0$ and $\theta_z(z = 0) = \theta_z(z = L_z) = 0$, which imply that $\sin(k_y L_y) = 0$ and $\sin(k_z L_z) = 0$. Therefore, $k_y = \frac{n_y\pi}{L_y}$ and $k_z = \frac{n_z\pi}{L_z}$ for $n_y, n_z \in \mathbb{Z}$. Without loss of generality, we restrict $n_y$ and $n_z$ to nonnegative integers. In addition, because $L_y$ and $L_z$ are finite, the minimum values of $k_y$ and $k_z$ are nonzero and are equal to $\frac{\pi}{L_y}$ and $\frac{\pi}{L_z}$ respectively. In summary, we conclude that $n_y, n_z \in \mathbb{Z}^+$, which is the set of positive integers.

### D. Constraints

For galvanostatic conditions,

$$\begin{aligned} I_\mathrm{a} &= L_y L_z \hat{n}\cdot J_0(x = h_0^\mathrm{c}) + \hat{n}\cdot J_1(x = h_0^\mathrm{c})\int_0^{L_y}\int_0^{L_z}\hat{\epsilon}^\mathrm{c}\,\mathrm{d}y\,\mathrm{d}z \\ &= -L_y L_z \hat{n}\cdot J_0(x = h_0^\mathrm{a}) - \hat{n}\cdot J_1(x = h_0^\mathrm{a})\int_0^{L_y}\int_0^{L_z}\hat{\epsilon}^\mathrm{a}\,\mathrm{d}y\,\mathrm{d}z \end{aligned} \tag{139}$$

where the "a" and "c" superscripts on $\hat{\epsilon}$ denote that the surface integrals involving $\hat{\epsilon}$ are performed over the anode and cathode respectively. Because $k_y = \frac{n_y\pi}{L_y}$ and $k_z = \frac{n_z\pi}{L_z}$ for $n_y, n_z \in \mathbb{Z}^+$, the surface integrals involving $\hat{\epsilon}$ are 0 and the constraint is automatically satisfied at $\mathcal{O}(\epsilon)$. At $\mathcal{O}(1)$, defining the dimensionless limiting current density $J_\mathrm{a}$ as $J_\mathrm{a} \equiv \frac{I_\mathrm{a}}{A} = \frac{I_\mathrm{a}}{L_y L_z}$,

$$\hat{n}\cdot J_0(x = h_0^\mathrm{c}) = -\hat{n}\cdot J_0(x = h_0^\mathrm{a}) = J_\mathrm{a}. \tag{140}$$

For potentiostatic conditions, $\phi_\mathrm{e}^\mathrm{c} = V$.

### E. Base state

At $\mathcal{O}(1)$, the governing PDEs are given by

$$c_{0,t} - D\left[c_{0,xx} + z(c_0\phi_{0,x})_x\right] = 0, \tag{141}$$

$$\beta_{\mathrm{D}}\left[(D - D_+)c_{0,xx} + z_+D_+\rho_{\mathrm{s}}\phi_{0,xx} - (z_+D_+ - zD)(c_0\phi_{0,x})_x\right] = 0. \tag{142}$$

The boundary conditions at $x = h_0^{\mathrm{a}}$ are given by

$$\phi_{\mathrm{e}}^{\mathrm{a}} = 0, \tag{143}$$

$$-D(-c_{0,x} - zc_0\phi_{0,x}) = 0, \tag{144}$$

$$\hat{n}\cdot J_0 = j_{0,0}\{\exp(-\alpha n\eta_0) - \exp[(1-\alpha)n\eta_0]\}, \tag{145}$$

$$-\dot{h}_0 = -\beta_{\mathrm{v}}\hat{n}\cdot J_0 + u_x. \tag{146}$$

The boundary conditions at $x = h_0^{\mathrm{c}}$ are given by

$$-D(c_{0,x} + zc_0\phi_{0,x}) = 0, \tag{147}$$

$$\hat{n}\cdot J_0 = j_{0,0}\{\exp(-\alpha n\eta_0) - \exp[(1-\alpha)n\eta_0]\}, \tag{148}$$

$$\dot{h}_0 = -\beta_{\mathrm{v}}\hat{n}\cdot J_0 - u_x. \tag{149}$$

We pick $u_x(x = h_0^{\mathrm{a}})$ and $u_x(x = h_0^{\mathrm{c}})$ such that the positions of the anode and cathode in the base state remain stationary, i.e., $\dot{h}_0^{\mathrm{a}} = \dot{h}_0^{\mathrm{c}} = 0$. Therefore, $u_x = \beta_{\mathrm{v}}\hat{n}\cdot J_0(x = h_0^{\mathrm{a}}) = -\beta_{\mathrm{v}}\hat{n}\cdot J_0(x = h_0^{\mathrm{c}})$ where the second equality automatically holds true because of charge conservation in the 1D $\mathcal{O}(1)$ base state. Physically, $u_x$ is equal to the velocity of the growing planar cathode/electrolyte interface or the dissolving planar anode/electrolyte interface in the base state. The initial conditions are given by

$$c_0(t = 0) = \beta_1, \tag{150}$$

$$h_0^{\mathrm{a}}(t = 0) = 0, \tag{151}$$

$$h_0^{\mathrm{c}}(t = 0) = 1. \tag{152}$$

Since $\dot{h}_0^{\mathrm{a}} = \dot{h}_0^{\mathrm{c}} = 0$, $h_0^{\mathrm{a}}(t) = 0$ and $h_0^{\mathrm{c}}(t) = 1$ for all $t$. For galvanostatic conditions,

$$J_{\mathrm{a}} = \beta_{\mathrm{D}}[(D - D_+)c_{0,x} + z_+D_+\rho_{\mathrm{s}}\phi_{0,x} - (z_+D_+ - zD)c_0\phi_{0,x}]|_{x=h_0^{\mathrm{c}}} \tag{153}$$

$$= \beta_{\mathrm{D}}[(D - D_+)c_{0,x} + z_+D_+\rho_{\mathrm{s}}\phi_{0,x} - (z_+D_+ - zD)c_0\phi_{0,x}]|_{x=h_0^{\mathrm{a}}}. \tag{154}$$

For potentiostatic conditions, $\phi_{\mathrm{e}}^{\mathrm{c}} = V$.

### F. Perturbed state

We first note that the PDEs given by Equations 141 and 142 apply at the $x = h_0^{\mathrm{a,c}}$ boundaries too. Therefore, at the anode,

$$\hat{n} \cdot F_1 = c_{0,t} h_1 - D[-c_1' - z(c_0 \phi_1' + \phi_{0,x} c_1)], \tag{155}$$

$$\hat{n} \cdot J_1 = \beta_{\mathrm{D}}[-(D - D_+)c_1' - z_+ D_+ \rho_{\mathrm{s}} \phi_1' + (z_+ D_+ - zD)(c_0 \phi_1' + \phi_{0,x} c_1)], \tag{156}$$

and at the cathode,

$$\hat{n} \cdot F_1 = -c_{0,t} h_1 - D[c_1' + z(c_0 \phi_1' + \phi_{0,x} c_1)], \tag{157}$$

$$\hat{n} \cdot J_1 = \beta_{\mathrm{D}}[(D - D_+)c_1' + z_+ D_+ \rho_{\mathrm{s}} \phi_1' - (z_+ D_+ - zD)(c_0 \phi_1' + \phi_{0,x} c_1)]. \tag{158}$$

At $\mathcal{O}(\epsilon)$, the governing ODEs (ordinary differential equations) are given by

$$D\big\{c_1'' - k^2 c_1 + z\big[(c_0 \phi_1' + \phi_{0,x} c_1)_x - k^2 c_0 \phi_1\big]\big\} = \omega c_1, \tag{159}$$

$$(D - D_+)\big(c_1'' - k^2 c_1\big) + z_+ D_+ \rho_{\mathrm{s}} \big(\phi_1'' - k^2 \phi_1\big) - (z_+ D_+ - zD)\big[(c_0 \phi_1' + \phi_{0,x} c_1)_x - k^2 c_0 \phi_1\big] = 0. \tag{160}$$

The boundary conditions at $x = h_0^{\mathrm{a}}$ are given by

$$c_{0,t} h_1^{\mathrm{a}} - D[-c_1' - z(c_0 \phi_1' + \phi_{0,x} c_1)] = 0, \tag{161}$$

$$\beta_{\mathrm{v}} j_{0,0} \Big(\hat{D}_1 h_1^{\mathrm{a}} + \hat{D}_2 c_1 + \hat{D}_3 \phi_1\Big) = \omega h_1^{\mathrm{a}}, \tag{162}$$

$$\beta_{\mathrm{m}}[-(D - D_+)c_1' - z_+ D_+ \rho_{\mathrm{s}} \phi_1' + (z_+ D_+ - zD)(c_0 \phi_1' + \phi_{0,x} c_1)] = \omega h_1^{\mathrm{a}}. \tag{163}$$

The boundary conditions at $x = h_0^{\mathrm{c}}$ are given by

$$-c_{0,t} h_1^{\mathrm{c}} - D[c_1' + z(c_0 \phi_1' + \phi_{0,x} c_1)] = 0, \tag{164}$$

$$\beta_{\mathrm{v}} j_{0,0} \Big(\hat{G}_1 h_1^{\mathrm{c}} + \hat{G}_2 c_1 + \hat{G}_3 \phi_1\Big) = -\omega h_1^{\mathrm{c}}, \tag{165}$$

$$\beta_{\mathrm{m}}[(D - D_+)c_1' + z_+ D_+ \rho_{\mathrm{s}} \phi_1' - (z_+ D_+ - zD)(c_0 \phi_1' + \phi_{0,x} c_1)] = -\omega h_1^{\mathrm{c}}. \tag{166}$$

## IV. DISCRETIZATION OF PERTURBED STATE

The 1D second-order accurate finite difference approximations for a uniform grid with a grid spacing $\Delta x$ are given by [3]

$$f_i' = \frac{f_{i+1} - f_{i-1}}{2\Delta x} + \mathcal{O}\big(\Delta x^2\big), \tag{167}$$

$$f_i' = \frac{-3f_i + 4f_{i+1} - f_{i+2}}{2\Delta x} + \mathcal{O}\big(\Delta x^2\big), \tag{168}$$

$$f_i' = \frac{f_{i-2} - 4f_{i-1} + 3f_i}{2\Delta x} + \mathcal{O}\big(\Delta x^2\big), \tag{169}$$

$$f_i'' = \frac{f_{i+1} - 2f_i + f_{i-1}}{\Delta x^2} + \mathcal{O}\big(\Delta x^2\big). \tag{170}$$

We pick a uniform grid and let $N$ be the number of grid points, therefore $\Delta x = \frac{1}{N-1}$. For brevity, we define the following dimensionless variables

$$\alpha_1 = D - D_+, \tag{171}$$

$$\alpha_2 = z_+ D_+ - zD. \tag{172}$$

We note that

$$\left(c_0\phi_1' + \phi_{0,x}c_1\right)_x - k^2 c_0\phi_1 = c_{0,x}\phi_1' + c_0\phi_1'' + \phi_{0,xx}c_1 + \phi_{0,x}c_1' - k^2 c_0\phi_1 \tag{173}$$

with the finite difference discretization

$$\begin{aligned}\left(c_0\phi_1' + \phi_{0,x}c_1\right)_{x,i} - k^2 c_{0,i}\phi_{1,i} = &\left(-\frac{\phi_{0,x,i}}{2\Delta x}\right)c_{1,i-1} + (\phi_{0,xx,i})c_{1,i} + \left(\frac{\phi_{0,x,i}}{2\Delta x}\right)c_{1,i+1} \\ &+ \left(-\frac{c_{0,x,i}}{2\Delta x} + \frac{c_{0,i}}{\Delta x^2}\right)\phi_{1,i-1} + \left(-\frac{2c_{0,i}}{\Delta x^2} - k^2 c_{0,i}\right)\phi_{1,i} + \left(\frac{c_{0,x,i}}{2\Delta x} + \frac{c_{0,i}}{\Delta x^2}\right)\phi_{1,i+1}.\end{aligned} \tag{174}$$

In addition,

$$\left(\theta_1'' - k^2\theta_1\right)_i = \left(\frac{1}{\Delta x^2}\right)\theta_{1,i-1} + \left(-\frac{2}{\Delta x^2} - k^2\right)\theta_{1,i} + \left(\frac{1}{\Delta x^2}\right)\theta_{1,i+1}. \tag{175}$$

The finite difference discretization of the $\mathcal{O}(\epsilon)$ equations in the domain results in

$$M_{1,i}c_{1,i-1} + M_{2,i}c_{1,i} + M_{3,i}c_{1,i+1} + M_{4,i}\phi_{1,i-1} + M_{5,i}\phi_{1,i} + M_{6,i}\phi_{1,i+1} = \omega c_{1,i}, \quad i = 2, \ldots, N-1, \tag{176}$$

$$M_{1,i} = D\left(\frac{1}{\Delta x^2} - z\frac{\phi_{0,x,i}}{2\Delta x}\right), \tag{177}$$

$$M_{2,i} = D\left(-\frac{2}{\Delta x^2} - k^2 + z\phi_{0,xx,i}\right), \tag{178}$$

$$M_{3,i} = D\left(\frac{1}{\Delta x^2} + z\frac{\phi_{0,x,i}}{2\Delta x}\right), \tag{179}$$

$$M_{4,i} = zD\left(-\frac{c_{0,x,i}}{2\Delta x} + \frac{c_{0,i}}{\Delta x^2}\right), \tag{180}$$

$$M_{5,i} = zD\left(-\frac{2c_{0,i}}{\Delta x^2} - k^2 c_{0,i}\right), \tag{181}$$

$$M_{6,i} = zD\left(\frac{c_{0,x,i}}{2\Delta x} + \frac{c_{0,i}}{\Delta x^2}\right), \tag{182}$$

$$A_{1,i}c_{1,i-1} + A_{2,i}c_{1,i} + A_{3,i}c_{1,i+1} + A_{4,i}\phi_{1,i-1} + A_{5,i}\phi_{1,i} + A_{6,i}\phi_{1,i+1} = 0, \quad i = 2, \ldots, N-1, \tag{183}$$

$$A_{1,i} = \alpha_1 \frac{1}{\Delta x^2} + \alpha_2 \frac{\phi_{0,x,i}}{2\Delta x}, \tag{184}$$

$$A_{2,i} = \alpha_1\left(-\frac{2}{\Delta x^2} - k^2\right) - \alpha_2 \phi_{0,xx,i}, \tag{185}$$

$$A_{3,i} = \alpha_1 \frac{1}{\Delta x^2} - \alpha_2 \frac{\phi_{0,x,i}}{2\Delta x}, \tag{186}$$

$$A_{4,i} = z_+ D_+ \rho_{\mathrm{s}} \frac{1}{\Delta x^2} - \alpha_2\left(-\frac{c_{0,x,i}}{2\Delta x} + \frac{c_{0,i}}{\Delta x^2}\right), \tag{187}$$

$$A_{5,i} = z_+ D_+ \rho_{\mathrm{s}}\left(-\frac{2}{\Delta x^2} - k^2\right) - \alpha_2\left(-\frac{2c_{0,i}}{\Delta x^2} - k^2 c_{0,i}\right), \tag{188}$$

$$A_{6,i} = z_+ D_+ \rho_{\mathrm{s}} \frac{1}{\Delta x^2} - \alpha_2\left(\frac{c_{0,x,i}}{2\Delta x} + \frac{c_{0,i}}{\Delta x^2}\right). \tag{189}$$

At the anode,

$$B_1 c_{1,1} + B_2 c_{1,2} + B_3 c_{1,3} + B_4 \phi_{1,1} + B_5 \phi_{1,2} + B_6 \phi_{1,3} = \omega h_1^{\mathrm{a}}, \tag{190}$$

$$B_1 = \beta_{\mathrm{m}}\left(\alpha_1 \frac{3}{2\Delta x} + \alpha_2 \phi_{0,x,1}\right), \tag{191}$$

$$B_2 = \beta_{\mathrm{m}}\left(-\alpha_1 \frac{2}{\Delta x}\right), \tag{192}$$

$$B_3 = \beta_{\mathrm{m}}\left(\alpha_1 \frac{1}{2\Delta x}\right), \tag{193}$$

$$B_4 = \beta_{\mathrm{m}}(\alpha_2 c_{0,1} - z_+ D_+ \rho_{\mathrm{s}})\left(-\frac{3}{2\Delta x}\right), \tag{194}$$

$$B_5 = \beta_{\mathrm{m}}(\alpha_2 c_{0,1} - z_+ D_+ \rho_{\mathrm{s}})\left(\frac{2}{\Delta x}\right), \tag{195}$$

$$B_6 = \beta_{\mathrm{m}}(\alpha_2 c_{0,1} - z_+ D_+ \rho_{\mathrm{s}})\left(-\frac{1}{2\Delta x}\right), \tag{196}$$

$$C_1 h_1^{\mathrm{a}} + C_2 c_{1,1} + C_3 c_{1,2} + C_4 c_{1,3} + C_5 \phi_{1,1} + C_6 \phi_{1,2} + C_7 \phi_{1,3} = 0, \tag{197}$$

$$C_1 = c_{0,t,1}, \tag{198}$$

$$C_2 = -D\left(\frac{3}{2\Delta x} - z\phi_{0,x,1}\right), \tag{199}$$

$$C_3 = -D\left(-\frac{2}{\Delta x}\right), \tag{200}$$

$$C_4 = -D\left(\frac{1}{2\Delta x}\right), \tag{201}$$

$$C_5 = zDc_{0,1}\left(-\frac{3}{2\Delta x}\right), \tag{202}$$

$$C_6 = zDc_{0,1}\left(\frac{2}{\Delta x}\right), \tag{203}$$

$$C_7 = zDc_{0,1}\left(-\frac{1}{2\Delta x}\right), \tag{204}$$

$$D_1 h_1^{\mathrm{a}} + D_2 c_{1,1} + D_3 \phi_{1,1} = \omega h_1^{\mathrm{a}}, \tag{205}$$

$$D_1 = \beta_{\mathrm{v}} j_{0,0,1} \hat{D}_1 = \beta_{\mathrm{v}} j_{0,0,1}\left[\alpha_{3,1} n\left(-\phi_{0,x,1} + \frac{\gamma k^2}{n}\right) + \frac{\exp(-\alpha n \eta_{0,1}) c_{0,x,1}}{c_{0,1} - \rho_{\mathrm{s}}}\right], \tag{206}$$

$$D_2 = \beta_{\mathrm{v}} j_{0,0,1} \hat{D}_2 = \beta_{\mathrm{v}} j_{0,0,1}\left[\frac{\exp(-\alpha n \eta_{0,1})}{c_{0,1} - \rho_{\mathrm{s}}}\right], \tag{207}$$

$$D_3 = \beta_{\mathrm{v}} j_{0,0,1} \hat{D}_3 = \beta_{\mathrm{v}} j_{0,0,1}(-\alpha_{3,1} n). \tag{208}$$

At the cathode,

$$E_1 c_{1,N-2} + E_2 c_{1,N-1} + E_3 c_{1,N} + E_4 \phi_{1,N-2} + E_5 \phi_{1,N-1} + E_6 \phi_{1,N} = -\omega h_1^{\mathrm{c}}, \tag{209}$$

$$E_1 = \beta_{\mathrm{m}}\left(\alpha_1 \frac{1}{2\Delta x}\right), \tag{210}$$

$$E_2 = \beta_{\mathrm{m}}\left(-\alpha_1 \frac{2}{\Delta x}\right), \tag{211}$$

$$E_3 = \beta_{\mathrm{m}}\left(\alpha_1 \frac{3}{2\Delta x} - \alpha_2 \phi_{0,x,N}\right), \tag{212}$$

$$E_4 = \beta_{\mathrm{m}}(\alpha_2 c_{0,N} - z_+ D_+ \rho_{\mathrm{s}})\left(-\frac{1}{2\Delta x}\right), \tag{213}$$

$$E_5 = \beta_{\mathrm{m}}(\alpha_2 c_{0,N} - z_+ D_+ \rho_{\mathrm{s}})\left(\frac{2}{\Delta x}\right), \tag{214}$$

$$E_6 = \beta_{\mathrm{m}}(\alpha_2 c_{0,N} - z_+ D_+ \rho_{\mathrm{s}})\left(-\frac{3}{2\Delta x}\right), \tag{215}$$

$$F_1 h_1^{\mathrm{c}} + F_2 c_{1,N-2} + F_3 c_{1,N-1} + F_4 c_{1,N} + F_5 \phi_{1,N-2} + F_6 \phi_{1,N-1} + F_7 \phi_{1,N} = 0, \tag{216}$$

$$F_1 = -c_{0,t,N}, \tag{217}$$

$$F_2 = -D\left(\frac{1}{2\Delta x}\right), \tag{218}$$

$$F_3 = -D\left(-\frac{2}{\Delta x}\right), \tag{219}$$

$$F_4 = -D\left(\frac{3}{2\Delta x} + z\phi_{0,x,N}\right), \tag{220}$$

$$F_5 = zDc_{0,N}\left(-\frac{1}{2\Delta x}\right), \tag{221}$$

$$F_6 = zDc_{0,N}\left(\frac{2}{\Delta x}\right), \tag{222}$$

$$F_7 = zDc_{0,N}\left(-\frac{3}{2\Delta x}\right), \tag{223}$$

$$G_1 h_1^{\mathrm{c}} + G_2 c_{1,N} + G_3 \phi_{1,N} = -\omega h_1^{\mathrm{c}}, \tag{224}$$

$$G_1 = \beta_{\mathrm{v}} j_{0,0,N} \hat{G}_1 = \beta_{\mathrm{v}} j_{0,0,N}\left[\alpha_{3,N} n\left(-\phi_{0,x,N} - \frac{\gamma k^2}{n}\right) + \frac{\exp(-\alpha n \eta_{0,N}) c_{0,x,N}}{c_{0,N} - \rho_{\mathrm{s}}}\right], \tag{225}$$

$$G_2 = \beta_{\mathrm{v}} j_{0,0,N} \hat{G}_2 = \beta_{\mathrm{v}} j_{0,0,N}\left[\frac{\exp(-\alpha n \eta_{0,N})}{c_{0,N} - \rho_{\mathrm{s}}}\right], \tag{226}$$

$$G_3 = \beta_{\mathrm{v}} j_{0,0,N} \hat{G}_3 = \beta_{\mathrm{v}} j_{0,0,N}(-\alpha_{3,N} n). \tag{227}$$

We can write all equations as the following generalized eigenvalue problem

$$Yv = \omega Zv, \tag{228}$$

$$v = \begin{bmatrix} h_1^{\mathrm{a}} \\ c_{1,1} \\ \phi_{1,1} \\ c_{1,2} \\ \phi_{1,2} \\ \vdots \\ c_{1,N-1} \\ \phi_{1,N-1} \\ c_{1,N} \\ \phi_{1,N} \\ h_1^{\mathrm{c}} \end{bmatrix} \in \mathbb{C}^{2N+2}, \tag{229}$$

$$
Y = \begin{bmatrix}
D_1 & D_2 & D_3 \\
C_1 & C_2 & C_5 & C_3 & C_6 & C_4 & C_7 \\
 & B_1 & B_4 & B_2 & B_5 & B_3 & B_6 \\
 & M_{1,2} & M_{4,2} & M_{2,2} & M_{5,2} & M_{3,2} & M_{6,2} \\
 & A_{1,2} & A_{4,2} & A_{2,2} & A_{5,2} & A_{3,2} & A_{6,2} \\
 & & & M_{1,3} & M_{4,3} & M_{2,3} & M_{5,3} & M_{3,3} & M_{6,3} \\
 & & & A_{1,3} & A_{4,3} & A_{2,3} & A_{5,3} & A_{3,3} & A_{6,3} \\
 & & & & & \ddots & \ddots & \ddots & \ddots & \ddots \ddots \\
 & & & & & \ddots & \ddots & \ddots & \ddots & \ddots \ddots \\
 & & & & & & & \ddots & \ddots & \ddots \ddots & \ddots & \ddots \\
 & & & & & & & \ddots & \ddots & \ddots \ddots & \ddots & \ddots \\
 & & & & & & & & & \ddots \ddots & \ddots & \ddots & \ddots & \ddots \\
 & & & & & & & & & \ddots \ddots & \ddots & \ddots & \ddots & \ddots \\
 & & & & & & & & & & M_{1,N-2} & M_{4,N-2} & M_{2,N-2} & M_{5,N-2} & M_{3,N-2} & M_{6,N-2} \\
 & & & & & & & & & & A_{1,N-2} & A_{4,N-2} & A_{2,N-2} & A_{5,N-2} & A_{3,N-2} & A_{6,N-2} \\
 & & & & & & & & & & & & M_{1,N-1} & M_{4,N-1} & M_{2,N-1} & M_{5,N-1} & M_{3,N-1} & M_{6,N-1} \\
 & & & & & & & & & & & & A_{1,N-1} & A_{4,N-1} & A_{2,N-1} & A_{5,N-1} & A_{3,N-1} & A_{6,N-1} \\
 & & & & & & & & & & & & E_1 & E_4 & E_2 & E_5 & E_3 & E_6 \\
 & & & & & & & & & & & & F_2 & F_5 & F_3 & F_6 & F_4 & F_7 & F_1 \\
 & & & & & & & & & & & & & & & & G_2 & G_3 & G_1
\end{bmatrix}
\in \mathbb{R}^{(2N+2)\times(2N+2)}, \tag{230}
$$

$$
Z = \begin{bmatrix}
1 & 0 & 0 \\
0 & 0 & 0 \\
1 & 0 & 0 \\
 & & & 1 \\
 & & & & 0 \\
 & & & & & 1 \\
 & & & & & & 0 \\
 & & & & & & & \ddots \\
 & & & & & & & & 1 \\
 & & & & & & & & & 0 \\
 & & & & & & & & & & 1 \\
 & & & & & & & & & & & 0 \\
 & & & & & & & & & & & & 0 & 0 & -1 \\
 & & & & & & & & & & & & 0 & 0 & 0 \\
 & & & & & & & & & & & & 0 & 0 & -1
\end{bmatrix}
\in \mathbb{R}^{(2N+2)\times(2N+2)}, \tag{231}
$$

where $Y, Z \in \mathbb{R}^{(2N+2)\times(2N+2)}$, $v \in \mathbb{C}^{2N+2}$ and $\omega \in \mathbb{C}$. $Y$ is non-singular with rank $2N+2$ and $Z$ is singular with rank $N$, therefore some of the eigenvalues are infinite. Since $v \in \mathbb{C}^{2N+2}$, the total number of eigenvalues is $2N+2$. $N$ eigenvalues are finite that correspond to the number of linearly independent rows/columns in $Z$, i.e., rank of $Z$, and $N+2$ eigenvalues are infinite that correspond to the number of linearly dependent rows/columns in $Z$. The linearly dependent rows/columns in $Z$ arise from the time-independent terms in the equations for the perturbed state.

While the ordering of the equations in $Y$ and $Z$ and variables in $v$ is natural and minimizes the bandwidths of $Y$ and $Z$, we would want to map the infinite eigenvalues to other arbitrarily chosen points in the complex plane [4] because we are only interested in the finite eigenvalues. To do so, we first subtract row 1 with row 3 and row $2N+2$ with row $2N$ so that rows 1 and $2N+2$ of $Z$ become zero rows:

$$D'_1 h_1^{\mathrm{a}} + D'_2 c_{1,1} + D'_3 c_{1,2} + D'_4 c_{1,3} + D'_5 \phi_{1,1} + D'_6 \phi_{1,2} + D'_7 \phi_{1,3} = 0, \tag{232}$$

$$D'_1 = D_1, \tag{233}$$

$$D'_2 = D_2 - B_1, \tag{234}$$

$$D'_3 = -B_2, \tag{235}$$

$$D'_4 = -B_3, \tag{236}$$

$$D'_5 = D_3 - B_4, \tag{237}$$

$$D'_6 = -B_5, \tag{238}$$

$$D'_7 = -B_6, \tag{239}$$

$$G'_1 h_1^{\mathrm{c}} + G'_2 c_{1,N-2} + G'_3 c_{1,N-1} + G'_4 c_{1,N} + G'_5 \phi_{1,N-2} + G'_6 \phi_{1,N-1} + G'_7 \phi_{1,N} = 0, \tag{240}$$

$$G'_1 = G_1, \tag{241}$$

$$G'_2 = -E_1, \tag{242}$$

$$G'_3 = -E_2, \tag{243}$$

$$G'_4 = G_2 - E_3, \tag{244}$$

$$G'_5 = -E_4, \tag{245}$$

$$G'_6 = -E_5, \tag{246}$$

$$G'_7 = G_3 - E_6. \tag{247}$$

Therefore, row 1 of $Y$ becomes

$$\begin{bmatrix} D'_1 & D'_2 & D'_5 & D'_3 & D'_6 & D'_4 & D'_7 & 0 & \cdots & 0 \end{bmatrix}, \tag{248}$$

while row $2N+2$ of $Y$ becomes

$$\begin{bmatrix} 0 & \cdots & 0 & G'_2 & G'_5 & G'_3 & G'_6 & G'_4 & G'_7 & G'_1 \end{bmatrix}. \tag{249}$$

By premultiplying $Z$ with a permutation matrix $P_\pi \in \mathbb{R}^{(2N+2)\times(2N+2)}$, we then permute $Z$ and accordingly $Y$ so that the $N+2$ zero rows in $Z$ are at the bottom. We denote the permuted $Y$ and $Z$ as $Y' \in \mathbb{R}^{(2N+2)\times(2N+2)}$ and $Z' \in \mathbb{R}^{(2N+2)\times(2N+2)}$ respectively and therefore, $Y' = P_\pi Y$ and $Z' = P_\pi Z$. The permutation matrix $P_\pi$ can be written as

$$P_\pi = \begin{bmatrix} e_{\pi(1)} \\ e_{\pi(2)} \\ \vdots \\ e_{\pi(2N+1)} \\ e_{\pi(2N+2)} \end{bmatrix} \tag{250}$$

where $e_i$ is the standard basis row vector of length $2N+2$ with 1 at its $i$-th entry and 0 everywhere else, and $\pi(\cdot)$ is the function that determines the order of permutation. In our case, $\pi(\cdot)$ is given by

$$\pi(1) = 3, \tag{251}$$

$$\pi(i) = 2i, \quad i = 2, \ldots, N-1, \tag{252}$$

$$\pi(N) = 2N, \tag{253}$$

$$\pi(N+1) = 1, \tag{254}$$

$$\pi(N+2) = 2, \tag{255}$$

$$\pi(i) = 2[i-(N+3)] + 5, \quad i = N+3, \ldots, 2N, \tag{256}$$

$$\pi(2N+1) = 2N+1, \tag{257}$$

$$\pi(2N+2) = 2N+2. \tag{258}$$

Following [4], we write $Y'$ and $Z'$ as

$$Y' = \begin{bmatrix} H \\ P \end{bmatrix}, \tag{259}$$

$$Z' = \begin{bmatrix} \hat{Z} \\ O \end{bmatrix}, \tag{260}$$

where $H \in \mathbb{R}^{N\times(2N+2)}$, $P \in \mathbb{R}^{(N+2)\times(2N+2)}$, $\hat{Z} \in \mathbb{R}^{N\times(2N+2)}$ is a matrix consisting of the nonzero rows of $Z'$, and $O \in \mathbb{R}^{(N+2)\times(2N+2)}$ is a zero matrix consisting of the zero rows of $Z'$. We define $E \in \mathbb{C}^{(N+2)\times(N+2)}$ as a diagonal matrix with entries $E_{ii} = -\sigma_i$ for $i = 1, \ldots, N+2$ where $\sigma_i \in \mathbb{C}$ is arbitrary and is the value that the $i$-th infinite eigenvalue is mapped to. The modified generalized eigenvalue problem then becomes

$$\bar{Y} v = \omega \bar{Z} v, \tag{261}$$

$$\bar{Y} = \begin{bmatrix} H \\ EP \end{bmatrix} \in \mathbb{R}^{(2N+2)\times(2N+2)}, \tag{262}$$

$$\bar{Z} = \begin{bmatrix} \hat{Z} \\ -P \end{bmatrix} \in \mathbb{R}^{(2N+2)\times(2N+2)}. \tag{263}$$

## V. PARAMETER SWEEPS

For various $\frac{t}{t_\mathrm{s}}$ values for $\rho_\mathrm{s} \in \{-0.05, 0, 0.05\}$ and $\mathrm{Da} \in \{0.1, 1, 10\}$, we plot numerically computed $\Re(\omega)$ against $k$ for $J_\mathrm{a} = 1$ (limiting current) in Figure 1 and $J_\mathrm{a} = 0.5$ (underlimiting current) in Figure 2.

## VI. BASE STATE ELECTRIC FIELD

We plot the dimensionless base state electric field $E_0$ against $x$ for various $\frac{t}{t_\mathrm{s}}$ values for $\rho_\mathrm{s} \in \{-0.05, 0, 0.05\}$ and $\mathrm{Da} \in \{0.1, 1, 10\}$ for $J_\mathrm{a} = 1.5$ (overlimiting current) in Figure 3, $J_\mathrm{a} = 1$ (limiting current) in Figure 4 and $J_\mathrm{a} = 0.5$ (underlimiting current) in Figure 5.

## VII. COMPARISON BETWEEN NUMERICAL AND APPROXIMATE SOLUTIONS

To illustrate how well the approximations given by Equations 49 and 50 in the main text work, for $\rho_\mathrm{s} \in \{-0.05, 0, 0.05\}$ and $\mathrm{Da} \in \{0.1, 1, 10\}$, we plot numerical and approximate values of $k_\mathrm{max}$ and $\omega_\mathrm{max}$ for $J_\mathrm{a} = 1.5$ in Figure 6, $J_\mathrm{a} = 1$ in Figure 7 and $J_\mathrm{a} = 0.5$ in Figure 8.

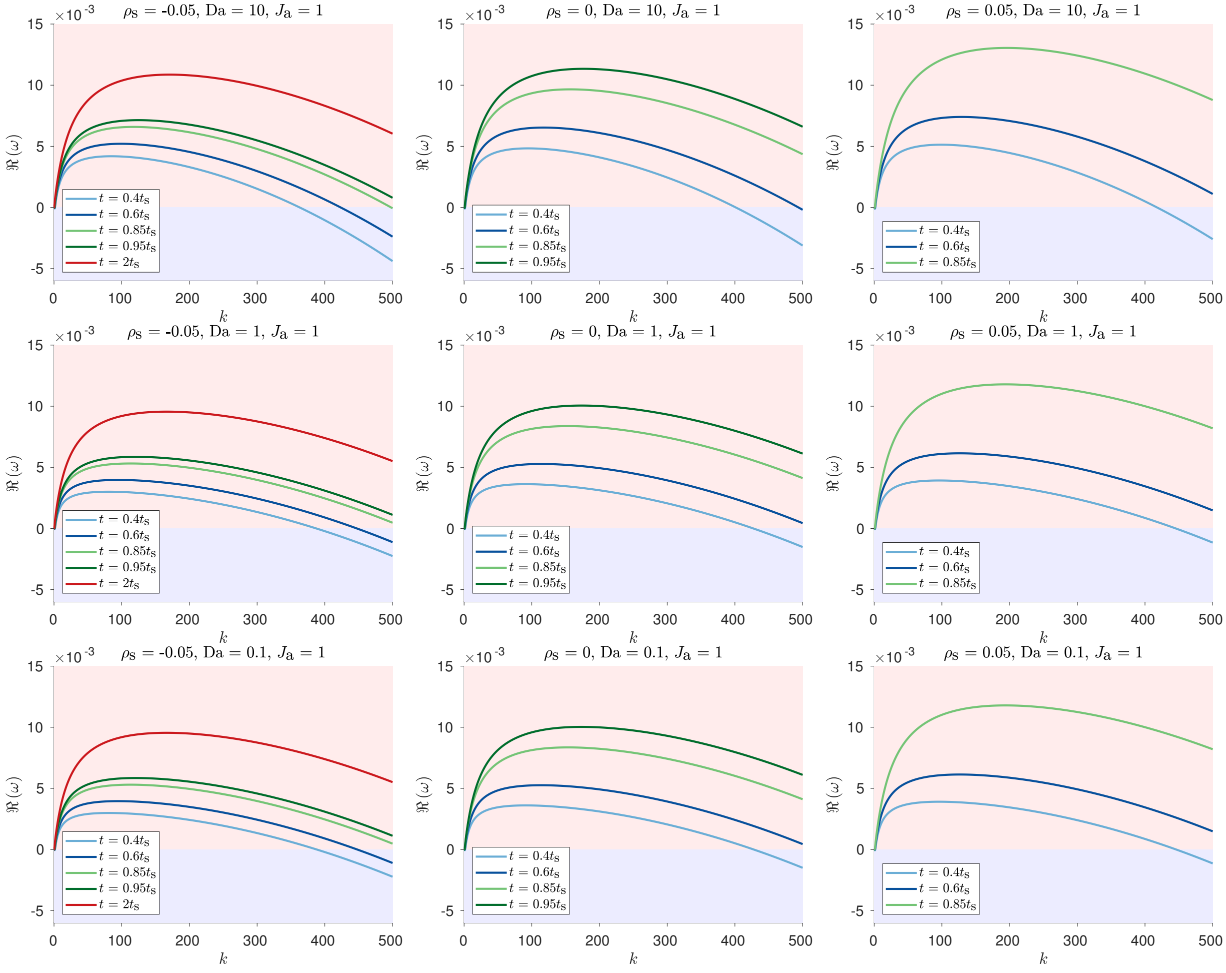


Figure 1. Plots of numerical $\Re(\omega)$ against $k$ for various $\frac{t}{t_s}$ values for $\rho_s \in \{-0.05, 0, 0.05\}$, Da $\in \{0.1, 1, 10\}$ and $J_a = 1$ (limiting current). $\rho_s$ increases from left to right and Da increases from bottom to top. Blue lines correspond to early times $t = 0.4t_s$ and $t = 0.6t_s$, green lines correspond to times near Sand's time $t = 0.85t_s$ and $t = 0.95t_s$, and red line corresponds to time beyond Sand's time $t = 2t_s$. For each color, intensity increases in the direction of increasing $t$.

For the same $\rho_s$ and Da ranges, we also plot numerical and approximate values of $k_c$ for $J_a = 1.5$ in Figure 9, $J_a = 1$ in Figure 10 and $J_a = 0.5$ in Figure 11.

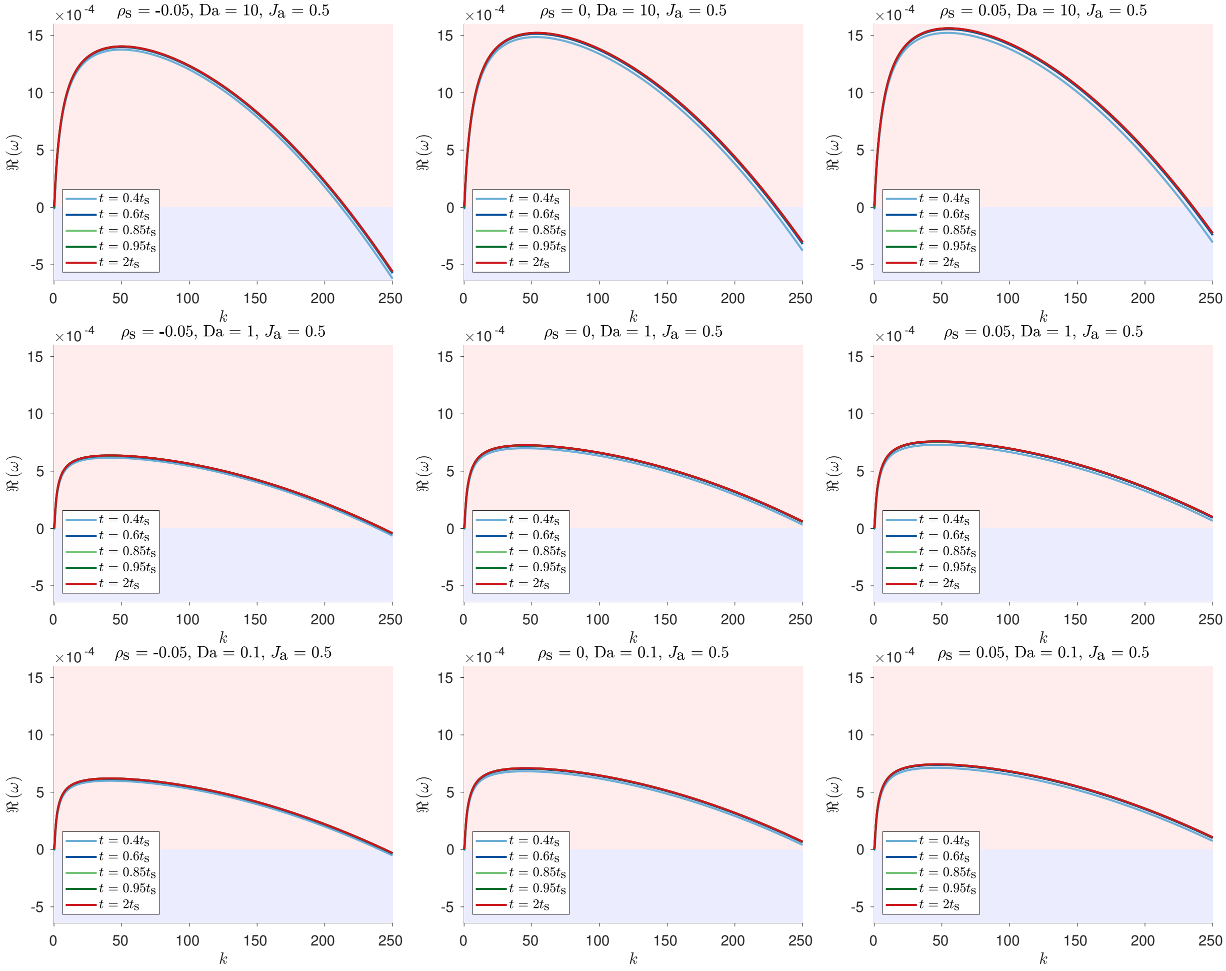


Figure 2. Plots of numerical $\Re(\omega)$ against $k$ for various $\frac{t}{t_{\mathrm{s}}}$ values for $\rho_{\mathrm{s}} \in \{-0.05, 0, 0.05\}$, $\mathrm{Da} \in \{0.1, 1, 10\}$ and $J_{\mathrm{a}} = 0.5$ (underlimiting current). $\rho_{\mathrm{s}}$ increases from left to right and Da increases from bottom to top. Blue lines correspond to early times $t = 0.4t_{\mathrm{s}}$ and $t = 0.6t_{\mathrm{s}}$, green lines correspond to times near Sand's time $t = 0.85t_{\mathrm{s}}$ and $t = 0.95t_{\mathrm{s}}$, and red line corresponds to time beyond Sand's time $t = 2t_{\mathrm{s}}$. For each color, intensity increases in the direction of increasing $t$.

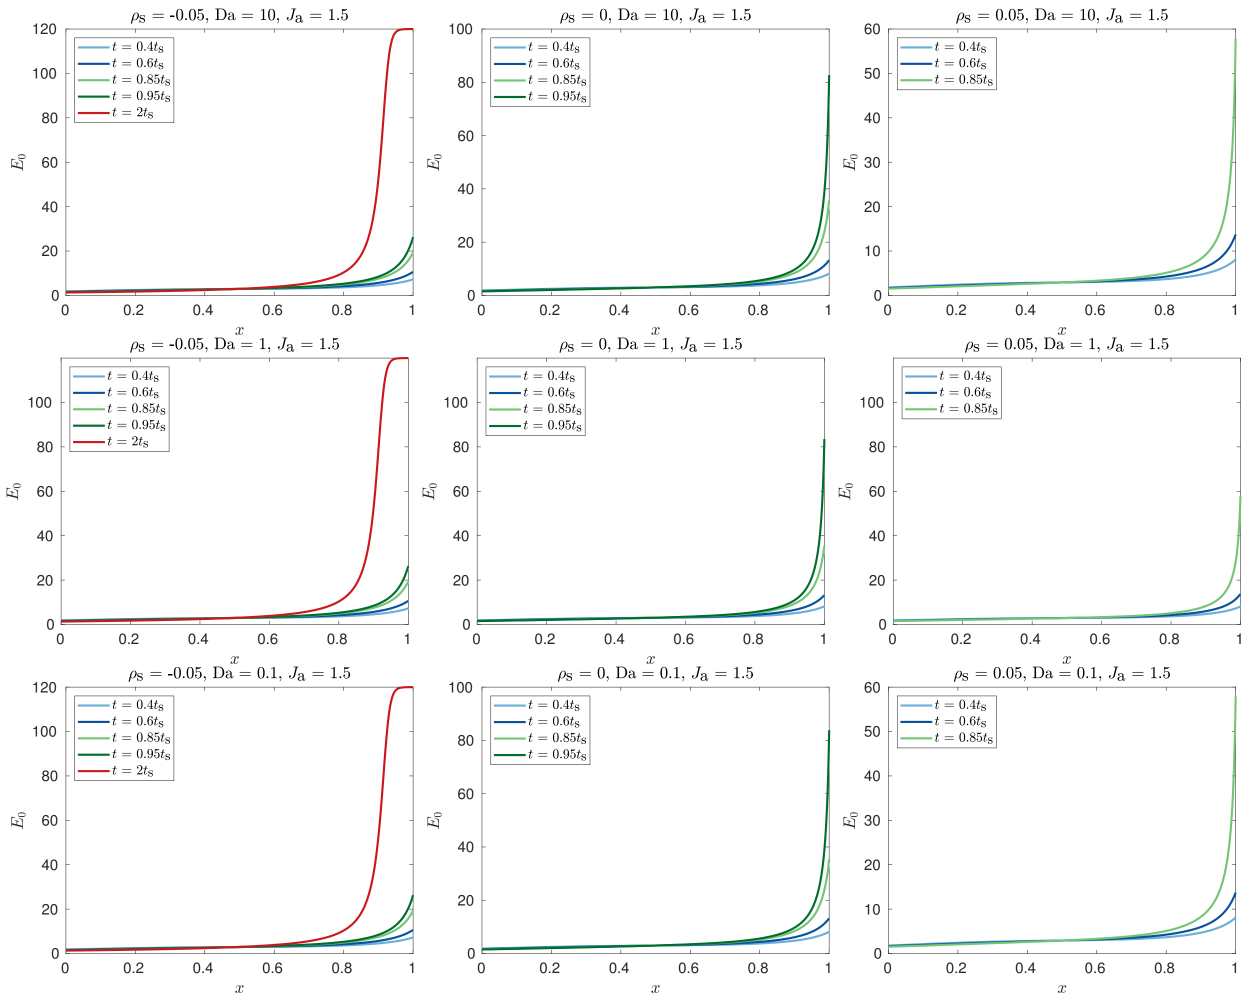


Figure 3. Plots of dimensionless base state electric field $E_0$ against $x$ for various $\frac{t}{t_s}$ values for $\rho_s \in \{-0.05, 0, 0.05\}$, Da $\in \{0.1, 1, 10\}$ and $J_a = 1.5$ (overlimiting current).

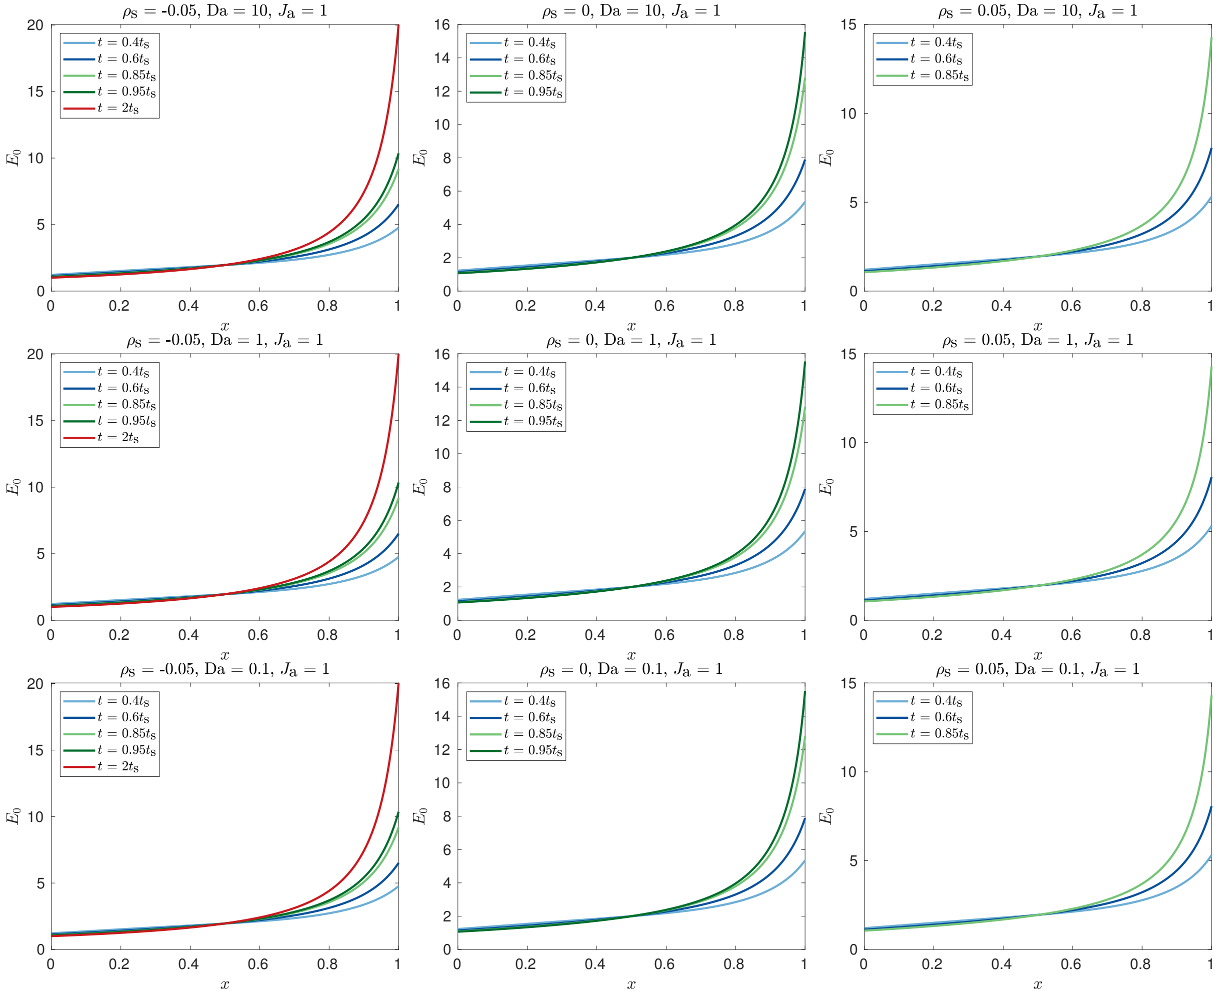


Figure 4. Plots of dimensionless base state electric field $E_0$ against $x$ for various $\frac{t}{t_s}$ values for $\rho_s \in \{-0.05, 0, 0.05\}$, $\mathrm{Da} \in \{0.1, 1, 10\}$ and $J_a = 1$ (limiting current).

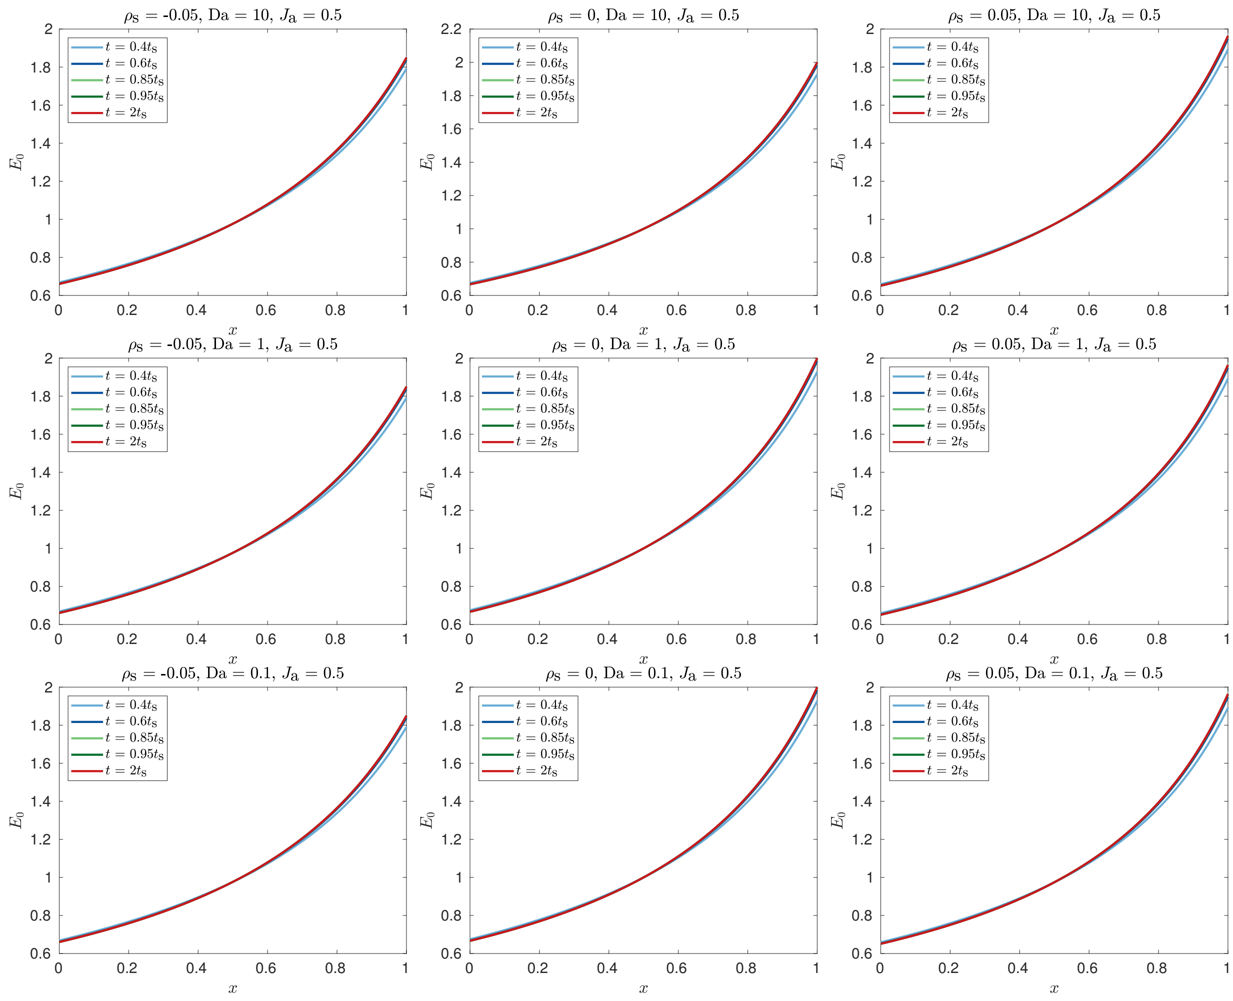

Figure 5. Plots of dimensionless base state electric field $E_0$ against $x$ for various $\frac{t}{t_s}$ values for $\rho_s \in \{-0.05, 0, 0.05\}$, $\mathrm{Da} \in \{0.1, 1, 10\}$ and $J_a = 0.5$ (underlimiting current).

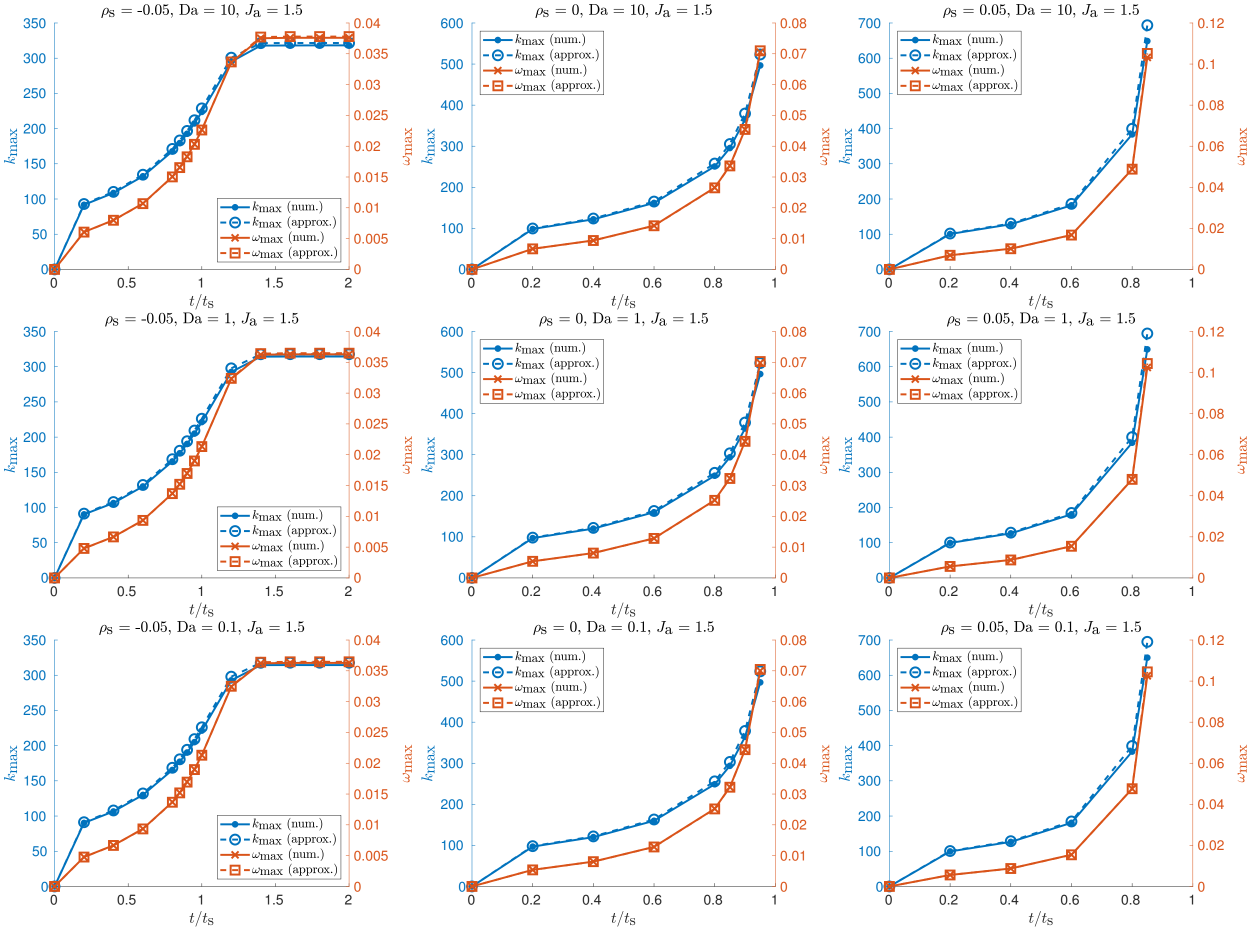


Figure 6. Plots of numerical and approximate values of $k_{\max}$ and $\omega_{\max}$ against $\frac{t}{t_s}$ for $\rho_s \in \{-0.05, 0, 0.05\}$, Da $\in \{0.1, 1, 10\}$ and $J_a = 1.5$ (overlimiting current). In the legends, "num." refers to numerical solutions while "approx." refers to approximate solutions.

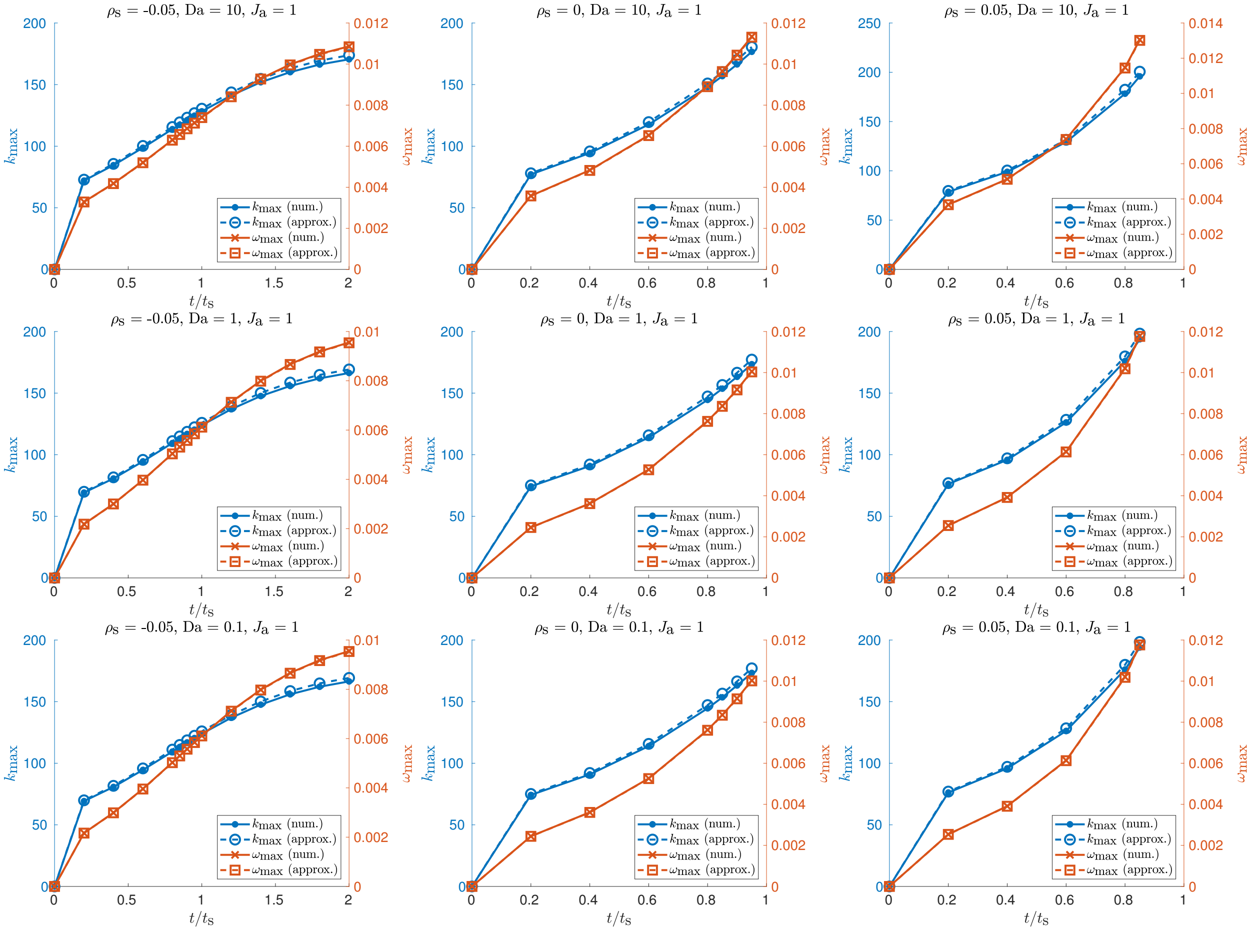


Figure 7. Plots of numerical and approximate values of $k_{\max}$ and $\omega_{\max}$ against $\frac{t}{t_s}$ for $\rho_s \in \{-0.05, 0, 0.05\}$, Da $\in \{0.1, 1, 10\}$ and $J_a = 1$ (limiting current). In the legends, "num." refers to numerical solutions while "approx." refers to approximate solutions.

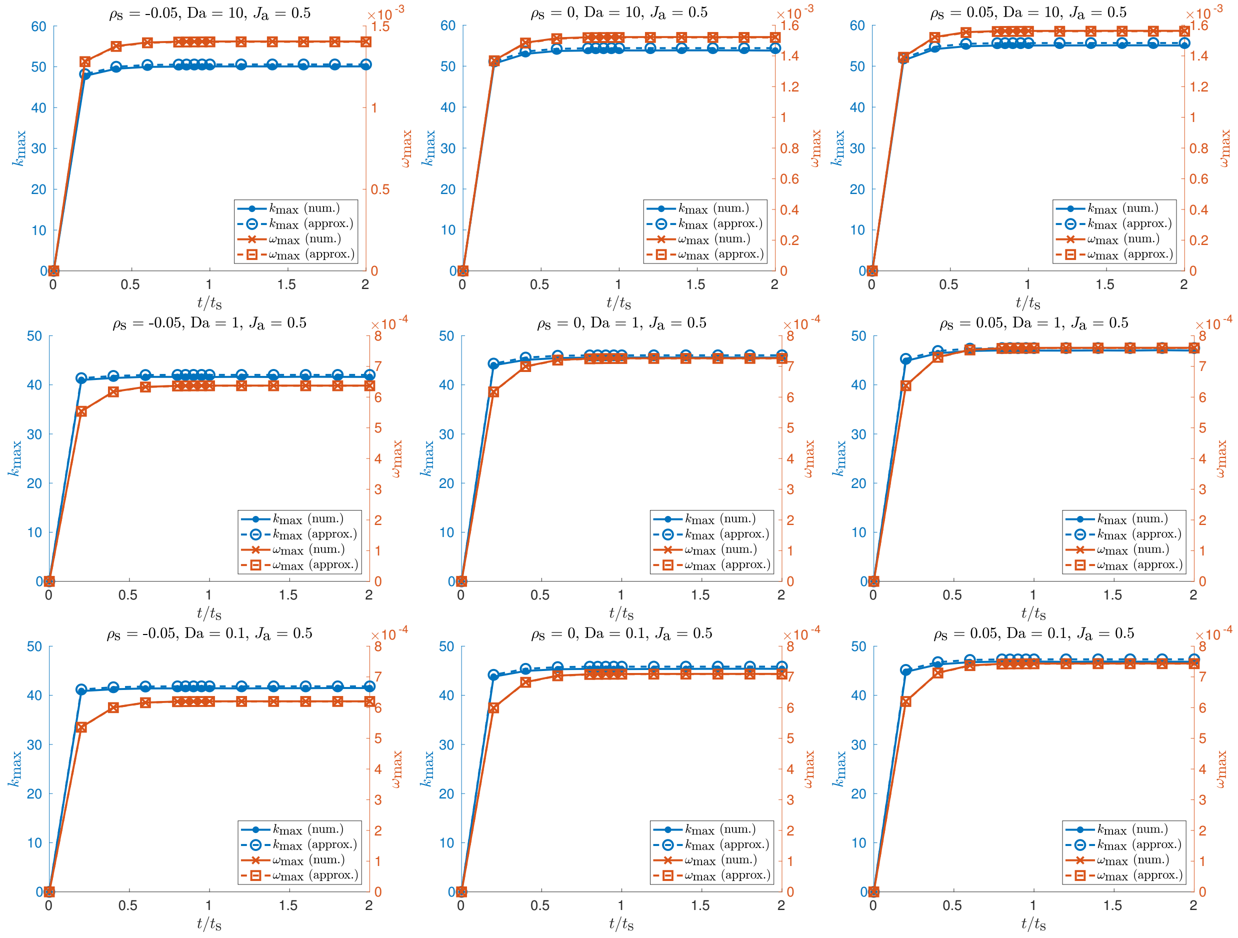

Figure 8. Plots of numerical and approximate values of $k_{\max}$ and $\omega_{\max}$ against $\frac{t}{t_s}$ for $\rho_s \in \{-0.05, 0, 0.05\}$, $\mathrm{Da} \in \{0.1, 1, 10\}$ and $J_a = 0.5$ (underlimiting current). In the legends, "num." refers to numerical solutions while "approx." refers to approximate solutions.

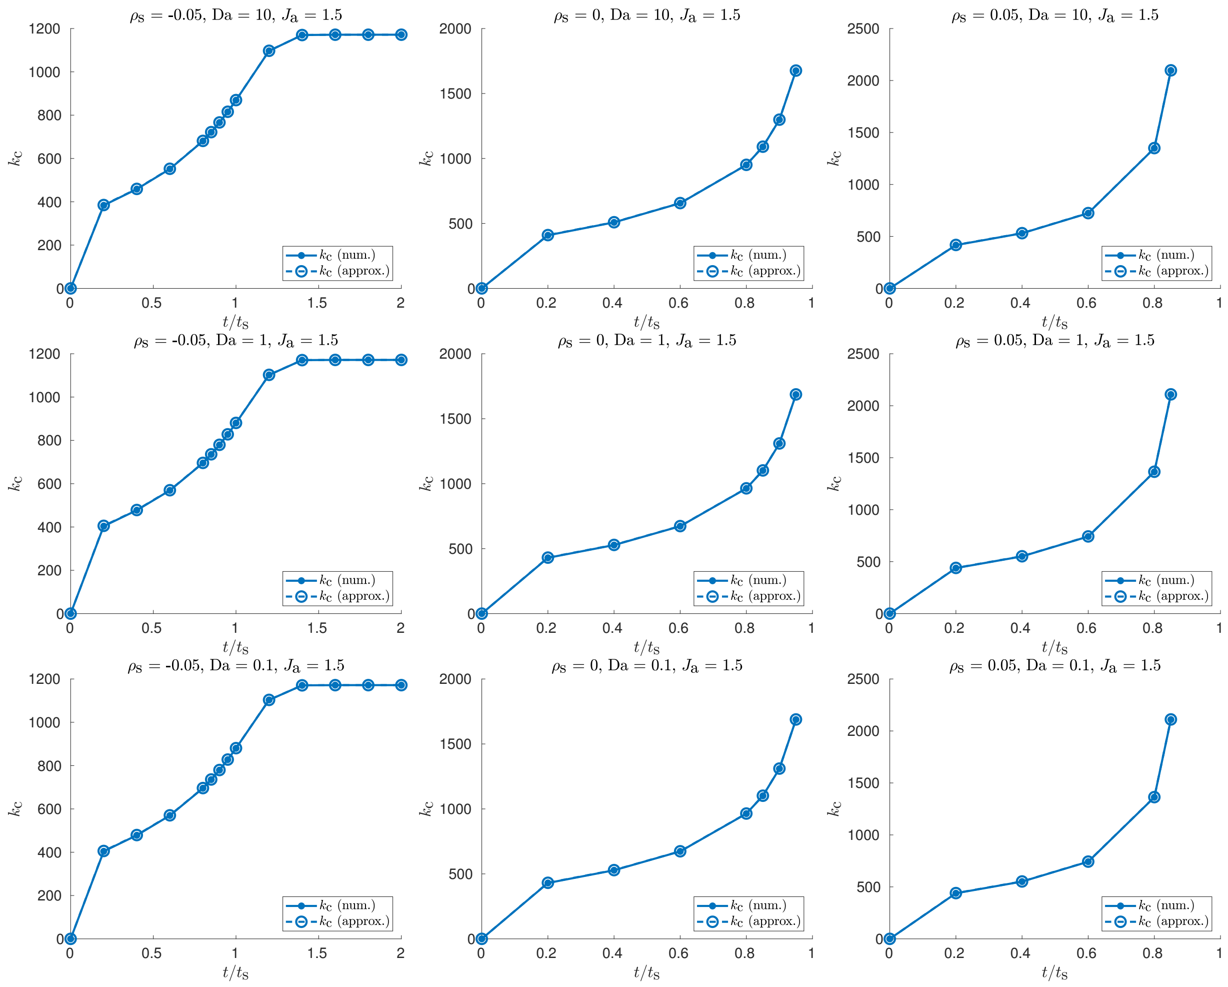


Figure 9. Plots of numerical and approximate values of $k_c$ against $\frac{t}{t_s}$ for $\rho_s \in \{-0.05, 0, 0.05\}$, $Da \in \{0.1, 1, 10\}$ and $J_a = 1.5$ (overlimiting current). In the legends, "num." refers to numerical solutions while "approx." refers to approximate solutions.

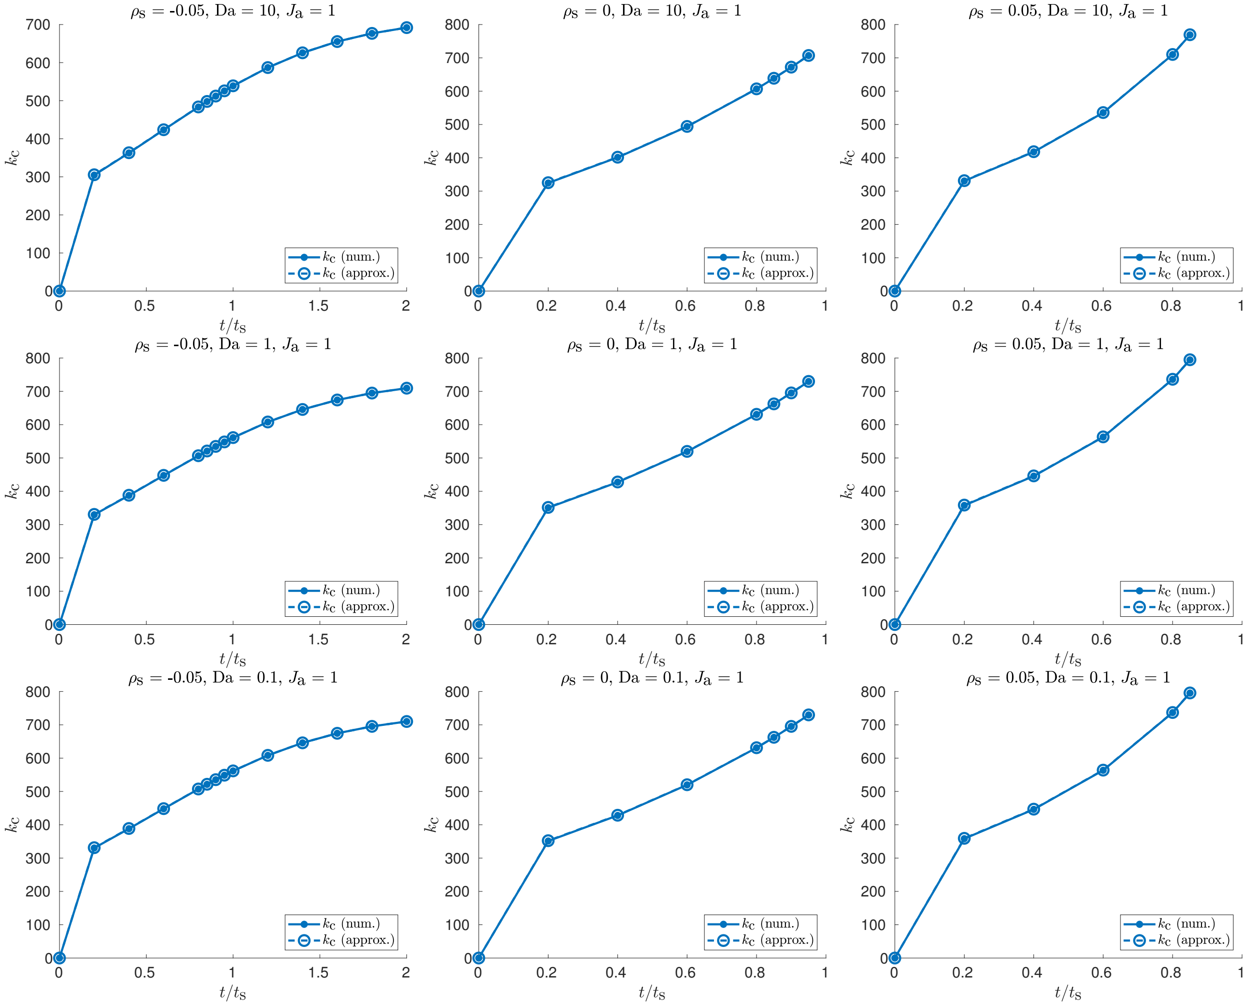


Figure 10. Plots of numerical and approximate values of $k_\mathrm{c}$ against $\frac{t}{t_\mathrm{s}}$ for $\rho_\mathrm{s} \in \{-0.05, 0, 0.05\}$, $\mathrm{Da} \in \{0.1, 1, 10\}$ and $J_\mathrm{a} = 1$ (limiting current). In the legends, "num." refers to numerical solutions while "approx." refers to approximate solutions.

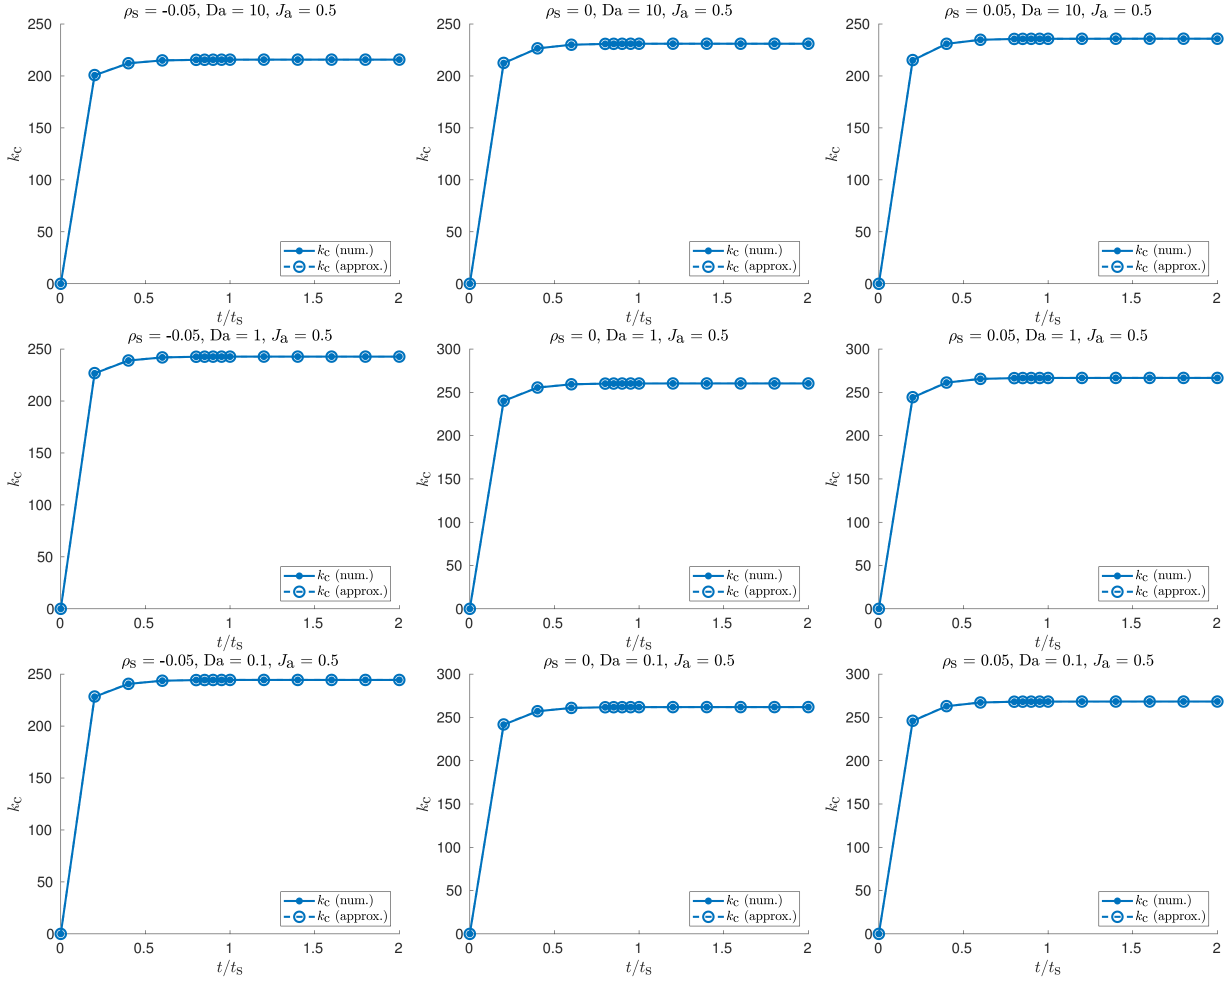


Figure 11. Plots of numerical and approximate values of $k_c$ against $\frac{t}{t_s}$ for $\rho_s \in \{-0.05, 0, 0.05\}$, $\mathrm{Da} \in \{0.1, 1, 10\}$ and $J_a = 0.5$ (underlimiting current). In the legends, "num." refers to numerical solutions while "approx." refers to approximate solutions.

[1] W. M. Deen, *Analysis of Transport Phenomena*, 2nd ed. (Oxford University Press, New York, 2011).

[2] J. Crank, *Free and Moving Boundary Problems* (Clarendon Press, Oxford Oxfordshire : New York, 1987).

[3] R. LeVeque, *Finite Difference Methods for Ordinary and Partial Differential Equations*, Other Titles in Applied Mathematics (Society for Industrial and Applied Mathematics, 2007).

[4] D. A. Goussis and A. J. Pearlstein, Journal of Computational Physics **84**, 242 (1989).
